# Supplementary material for: Core-set Sampling for Efficient Neural Architecture Search
Source: arXiv:2107.06869 source file (2021-07-08)
Supplement: Supplementary file 1 [file 7_Supplementary.tex]

%\onecolumn[
%\icmltitle{Appendix: Selective Focusing Learning in Conditional GANs}
%]

\appendix
\addcontentsline{toc}{section}{Appendices}
% \counterwithin*{equation}{part}
\setcounter{equation}{0}
\section{Connection to Other Methods}
\label{Connection to Other Methods}
We examined the compatibility of the proposed method with recent training methods for GANs. The experiments were conducted with the datasets that each method mainly used (ImageNet $64\times64$ and CIFAR-10). 

\textbf{Instance selection for GANs}
\citep{devries2020instance} analyzes instance selection \citep{olvera2010review} in the conditional generative setting. This method removes low density regions from the data manifold prior to model optimization. It improves the overall image sample quality in exchange for reducing diversity with a small model capacity and training time. By redefining target distribution through instance selection, SFL can be applied to easy target distribution. In this case, the proposed SFL is still effective because there are easy and hard samples in the new target distribution. We applied SFL and SFL+ to the dataset after instance selection. 
In Table \ref{Instance_SFL}, SFL+ outperformed the baseline for almost all metrics. Because the goal of instance selection is to remove low density regions, it is reasonable to say that the effectiveness of SFL reduced as the retention ratio (RR) reduced. Nevertheless, our SFL+ achieved a value that is $0.36$ lower than the best FID in instance selection.

\begin{table*}[h]
\centering

\caption{Performance on instance selected ImageNet $64\times64$ with the SA-GAN \cite{zhang2019self}. The RR and FR are the retention ratio (percentage of remaining dataset after instance selection) and maximum focusing ratio (maximum focusing rate of the remaining datasets), respectively. Best results in bold. $^{\ddagger}$ is quoted from \citep{devries2020instance}.}
% \vspace*{0.1in}
% \vskip -0.1in
\label{Instance_SFL}
\begin{tabular}{ccc|cccccc}
\Xhline{2\arrayrulewidth}
\begin{tabular}[c]{@{}c@{}}RR\\ (\%)\end{tabular} & Method & \begin{tabular}[c]{@{}c@{}}FR\\ (\%)\end{tabular} & IS $\uparrow$   & FID $\downarrow$  & P $\uparrow$ & R $\uparrow$   & D $\uparrow$   & C $\uparrow$   \\ \hline
\multirow{3}{*}{80}                               & Instance Selection$^{\ddagger}$   & 0                                               & 21.62 & 13.17 & 0.74 & \textbf{0.65} & 0.87 & 0.79 \\
                                                  & SFL     & 50                                                &   24.06    &   12.37    &  0.75    &  \textbf{0.65}    &   0.91  &   0.83   \\
                                                  & SFL+    & 50                                                &   \textbf{26.67}    & \textbf{11.29}      & \textbf{0.76}     & \textbf{0.65}     & \textbf{0.97}     & \textbf{0.85}     \\ \hline
\multirow{3}{*}{60}                               & Instance Selection$^{\ddagger}$   & 0                                               & 27.95 & 10.35 & 0.78 & \textbf{0.63} & 0.99 & 0.87 \\
                                                  & SFL     & 33                                                &   30.17    &   9.84    &  0.78    &   \textbf{0.63}   &   1.02   &   0.88   \\
                                                  & SFL+    & 33                                                &    \textbf{33.38}   & \textbf{8.79}      & \textbf{0.80}     &    \textbf{0.63}  & \textbf{1.12}     & \textbf{0.90}     \\ \hline
\multirow{3}{*}{40}                               & Instance Selection$^{\ddagger}$   & 0                                               & 37.10 & 9.07  & 0.81 & \textbf{0.60} & 1.12 & 0.90 \\
                                                  & SFL     & 12.5                                                &    37.52   &   8.87    &  0.82    &   \textbf{0.60}   &   1.16   &  0.91    \\
                                                  & SFL+    & 12.5                                                &    \textbf{40.65}   &   \textbf{8.71}    &  \textbf{0.83}    &   0.59   &   \textbf{1.20}   &   \textbf{0.92}   \\ \Xhline{2\arrayrulewidth}
\end{tabular}
\vskip -0.1in
\end{table*}

\textbf{The top-k training of GANs}
is a simple modification to the GAN training algorithm, improving performance by removing bad samples \citep{sinha2020top}. Since SFL also generates bad samples during the training, top-k can improve the performance of SFL. In Table \ref{Top-k training}, the top-k BigGAN outperformed the baseline BigGAN in all metrics except for Precision and Density. Further, SFL achieved better performance than top-k, and we can achieve state-of-the-art performance by applying both methods. 

\begin{table}[H]
\vskip -0.1in
\centering
\caption{Comparison to the top-k training of GANs on CIFAR-10. For a simple comparison, we set the maximum FR to $50\%$. $^{\ddagger}$ and $^{\dagger}$ are quoted from \citep{zhao2020feature} and \citep{wang2018improving}, respectively.}
\vspace*{0.1in}
\label{Top-k training}
\scalebox{0.91}{
\begin{tabular}{c|cccccc}
\Xhline{2\arrayrulewidth}
              Method   &   IS $\uparrow$    & FID $\downarrow$  & P $\uparrow$  & R $\uparrow$ & D $\uparrow$ & C $\uparrow$ \\ \hline
SN-GAN$^{\ddagger}$ &   8.22   &  14.26     & - &   -  & -   &  - \\ 
R-MMD-GAN$^{\dagger}$&   8.29   &  16.21     & - &  -  & -   &  - \\ 
BigGAN &   8.43   &  6.45     & \textbf{0.76} &   0.65  & 1.01   &  0.88 \\ 
FQ-BigGAN$^{\ddagger}$ &   8.48   &  5.59   & - &  -  & - & - \\ \hline
Top-k BigGAN  &   8.45   &  6.04     & 0.75 &  0.66  & 0.98 & 0.89 \\
SFL BigGAN &   8.60   &   5.89     & \textbf{0.76} &  0.66  & 1.01 &  0.91 \\
Both BigGAN&   \textbf{8.78}   &  \textbf{5.25}     & \textbf{0.76} &  \textbf{0.67}  & \textbf{1.02} & \textbf{0.92} \\
\Xhline{2\arrayrulewidth}
\end{tabular}}
\vskip -0.1in
\end{table}
\section{Exact Conditional Term for Projection Discriminator}
\label{sup_Exact_conditional_term}
% \counterwithin*{equation}{subsection}
In \citep{miyato2018project}, if $y$ is a categorical variable taking a value in $\{1,\cdots,C\}$ and $p_{data}(y|x)$ is obtained ising the softmax function, log $p_{data}(y=c|x)$ is represented by the following:
\begin{equation}
\log p_{data}(y=c|x):= (v_c^p)^{\text{T}}\phi(x)-\log Z^p(\phi(x)),
\label{eq:appen1}
\end{equation}
where $Z^p(\phi(x)):=\left(\sum_{j=1}^{C}\exp{\left((v_c^p)^{\text{T}}\phi(x)\right)}\right)$ is the normalization constant and is input into the final layer of the network model. If we parametrize the target distribution $p_g(y=c|x)$ in this form with the same choice of $\phi$, the log likelihood ratio $r(y|x)$ takes the following form:
\begin{multline}
\log \frac{p_{data}(y=c|x)}{p_g(y=c|x)}:= (v_c^p-v_c^g)^{\text{T}}\phi(x)\\ -(\log Z^p(\phi(x))-\log Z^g(\phi(x))).
\label{eq:appen2}
\end{multline}
Then, if $\mathbf{y}$ denotes a one-hot vector of the label $y$ and $V^p$ and $V^g$ denote the embedding matrices consisting of row vectors $v_c^p$ and $v_c^g$, we can rewrite the above equation:
\begin{multline}
D(y|x):= \mathbf{y}^{\text{T}}(V^p-V^g)\phi(x)\\-\underbrace{(\log Z^p(\phi(x))-\log Z^g(\phi(x)))}_{\text{normalization constant}}.
\label{eq:appen3}
\end{multline}
For efficient computation, the original projection discriminator \citep{miyato2018project} integrates $(V^p-V^g)$ into a single embedding matrix $V$ because it can put the normalization constant $(\log Z^p(\phi(x))-\log Z^g(\phi(x)))$ and marginal term $D(x)$ together into one expression $\psi(\phi(x))$. However, because SFL exploits only the conditional term to focus on easy samples, the normalization constant should be separated from the marginal term, and two embedding matrices are necessary. In Table \ref{Training time}, Exact SFL+ took $32.7\%$ more time than the approximated method due to adding the normalization constant and embedding matrix.

\section{Experiment Setup for Section \ref{Experiments}}
\label{sup_Experiment setup for Section}
\subsection{CIFAR-10 ($32\times32$)}
Parameters are set as follows: $bs = 50$, $ch =64$, $G\_lr = 2e^{-4}$, $D\_lr = 2e^{-4}$, $G\_step = 1$, $D\_step=4$ and $num\_epochs = 500$. In experiments on CIFAR-10 (Table \ref{Top-k training}), we set the maximum focusing ratio (FR) $\nu$ to $50\%$ ($\gamma=\nu^{(1/E_{max})}=0.5^{(1/500)}$).

\subsection{ImageNet ($64\times64$)}
For all experiments in Table \ref{various GAN architectures}, we set the maximum FR $\nu$ to $50\%$ ($\gamma=\nu^{(1/E_{max})}=0.5^{(1/50)}$). The remaining parameters are as follows:

SN-GAN: $bs = 64$, $ch =64$, $G\_attn = 0$, $D\_attn = 0$, $G\_lr = 2e^{-4}$, $D\_lr = 2e^{-4}$, $G\_step = 1$, $D\_step=5$ and $num\_iters = 500000$. 

SA-GAN: $bs = 128$, $ch =32$, $G\_attn = 32$, $D\_attn = 32$, $G\_lr = 1e^{-4}$, $D\_lr = 4e^{-4}$, $G\_step = 1$, $D\_step=1$ and $num\_iters = 500000$.

BigGAN: $bs = 128$, $ch =64$, $G\_attn = 64$, $D\_attn = 64$, $dim\_z  = 120$, $shared\_dim = 128$, $G\_lr = 1e^{-4}$, $D\_lr = 4e^{-4}$, $G\_step = 1$, $D\_step=1$ and $num\_iters = 500000$.

\begin{figure}[t]
\vskip -0.1in
\begin{center}
\centerline{\includegraphics[width=0.66\columnwidth]{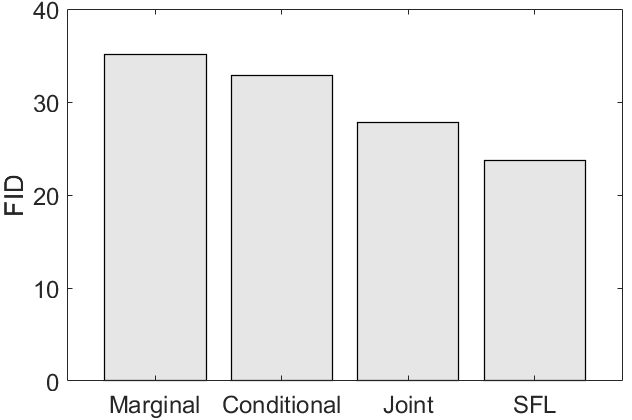}}
\vskip -0.15in
\caption{
Quantitative results for each matching. FID in the SA-GAN trained on ImageNet (\textbf{$64\times64$}) for each matching (for FID, a lower value is better).}
\label{Toy_FID_score}
\end{center}
\vskip -0.2in
\end{figure}

\section{Additional Results}
\label{Additional results}

\subsection{Generated Image Samples on ImageNet ($64\times64$)}
To verify the effectiveness of enforcing the conditional terms for easy samples, we first randomly generated image samples for a certain class and sorted the samples using the scoring function in \citep{devries2020instance}.  In Fig. \ref{visualization_SFL_sup}, In (a)-(d), we compared the samples corresponding to the red box of other classes and obtained similar results.

\begin{figure*}[h]
\centering
\subfigure[W/O SFL+ (Class 127)]{
\includegraphics[width=\columnwidth]{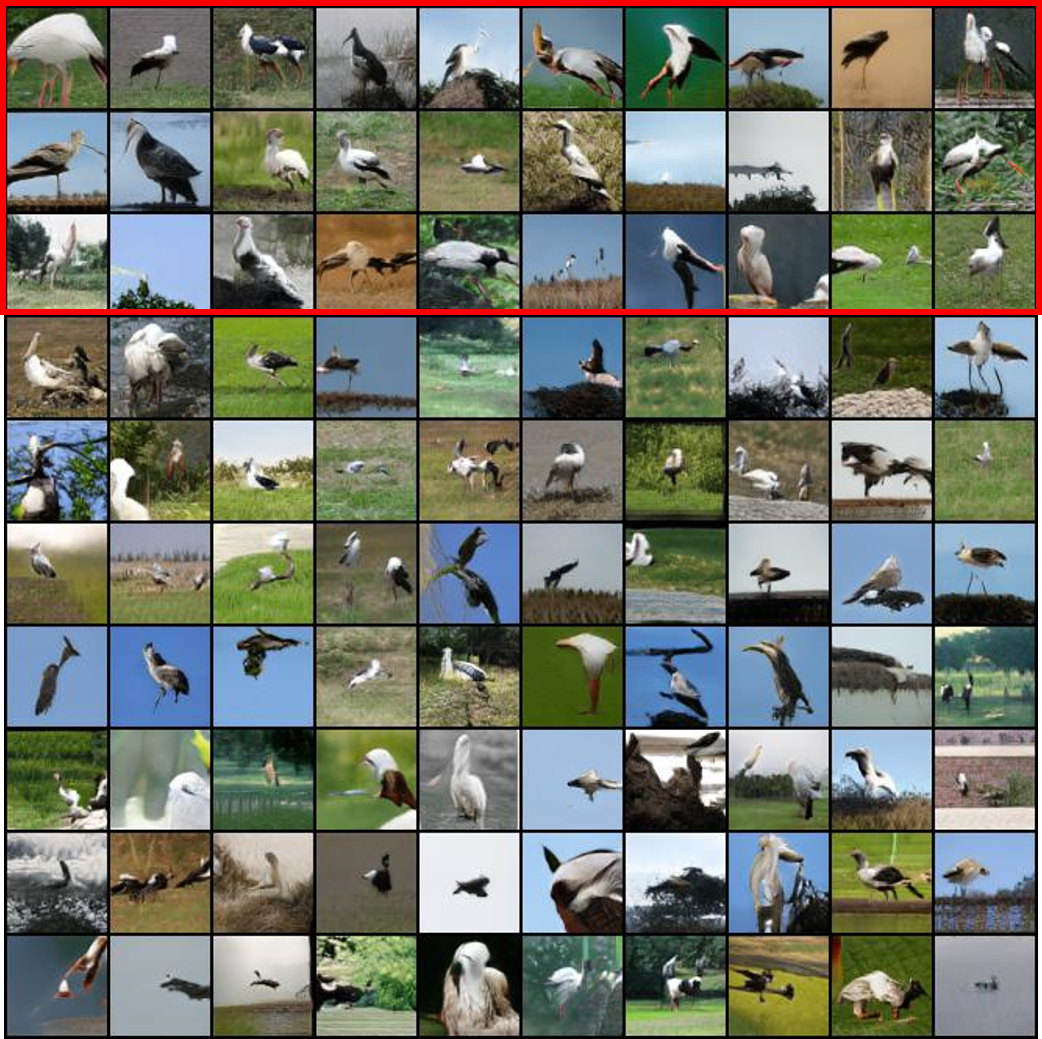}
\label{fig:without SFL}
}
\subfigure[W/ SFL+ (Class 127)]{
\includegraphics[width=\columnwidth]{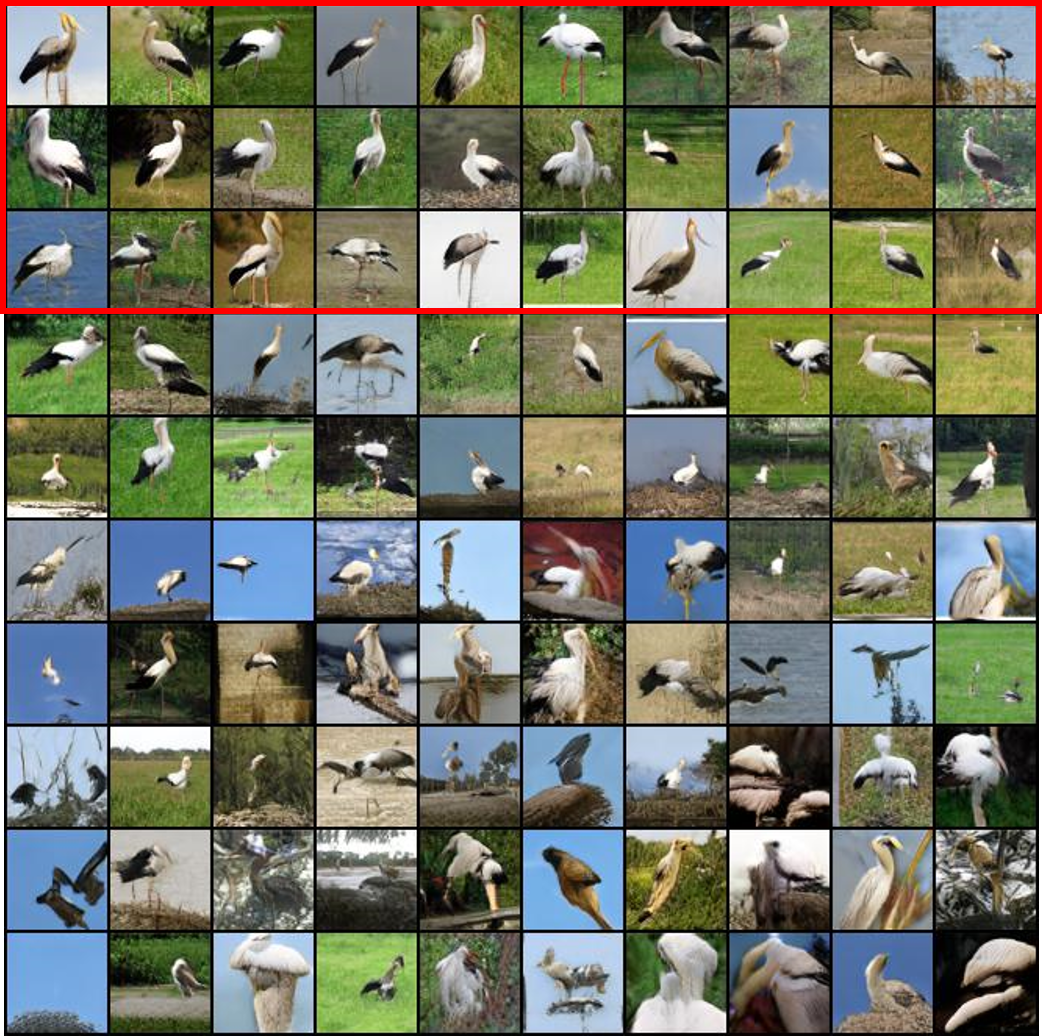}
\label{fig:with SFL}
}
\subfigure[W/O SFL+ (Class 243)]{
\includegraphics[width=\columnwidth]{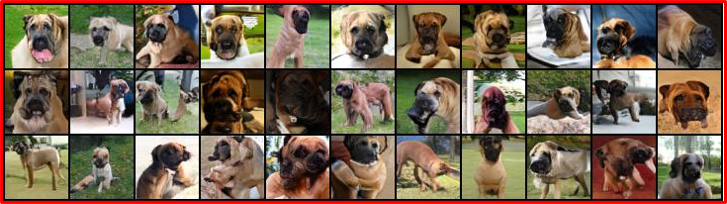}
\label{fig:without SFL}
}
\subfigure[W/ SFL+ (Class 243)]{
\includegraphics[width=\columnwidth]{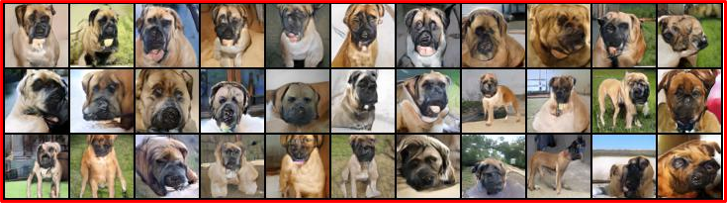}
\label{fig:with SFL}
}
\subfigure[W/O SFL+ (Class 374)]{
\includegraphics[width=\columnwidth]{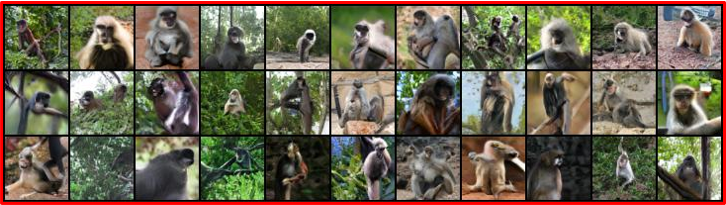}
\label{fig:without SFL}
}
\subfigure[W/ SFL+ (Class 374)]{
\includegraphics[width=\columnwidth]{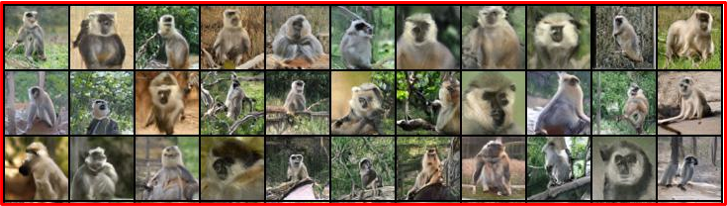}
\label{fig:with SFL}
}\vskip -0.1in
\subfigure[W/O SFL+ (Class 382)]{
\includegraphics[width=\columnwidth]{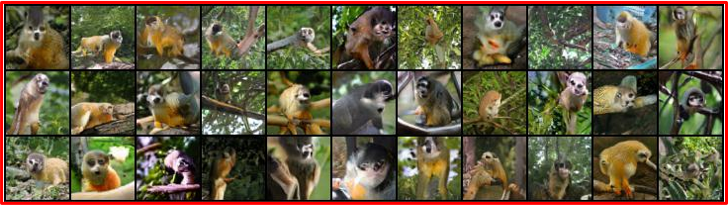}
\label{fig:without SFL}
}
\subfigure[W/ SFL+ (Class 382)]{
\includegraphics[width=\columnwidth]{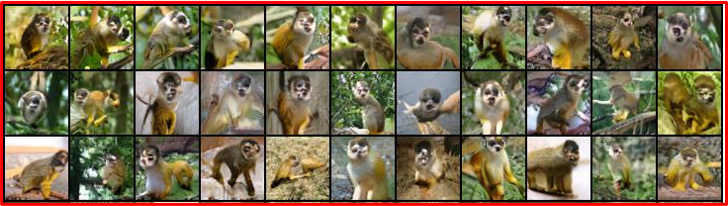}
\label{fig:with SFL}
}
\vskip -0.15in
\caption{
Comparison of the generated samples with and without SFL+ on ImageNet $64\times64$. (a), (b) Full generated samples sorted by easy to hard using the scoring function in \citep{devries2020instance}. (c), (d) Samples corresponding to the red box for class 243. (e), (f) Samples corresponding to the red box for class 374. (g), (h) Samples corresponding to the red box for class 382. Overall, SFL+ effectively learned the easy samples (red box) of the dataset.
}
\label{visualization_SFL_sup}
\vskip -0.2in
\end{figure*}

\subsection{Which data and players to apply SFL?}
%\label{Which data/player to apply SFL}
Next, we analyzed the effect of applying SFL to real and generated data. In Fig. \ref{supple effect of dtatplayer}, when the discriminator was learned by applying SFL only to the real data, the performance of the IS and FID degraded. The discriminator only accelerates the learning of easy samples, and the generator cannot be effectively enforced to learn these samples, causing overfitting of the discriminator. However, when the discriminator is learned by applying SFL to both the real and generated samples, it is possible to enforce the generator to learn easy samples, improving the fidelity and diversity compared to the baseline. Finally, when SFL is applied to the generator, we can achieve additional performance improvement.

\begin{figure*}[h]
\centering
\subfigure[]{
\includegraphics[width=.6\columnwidth]{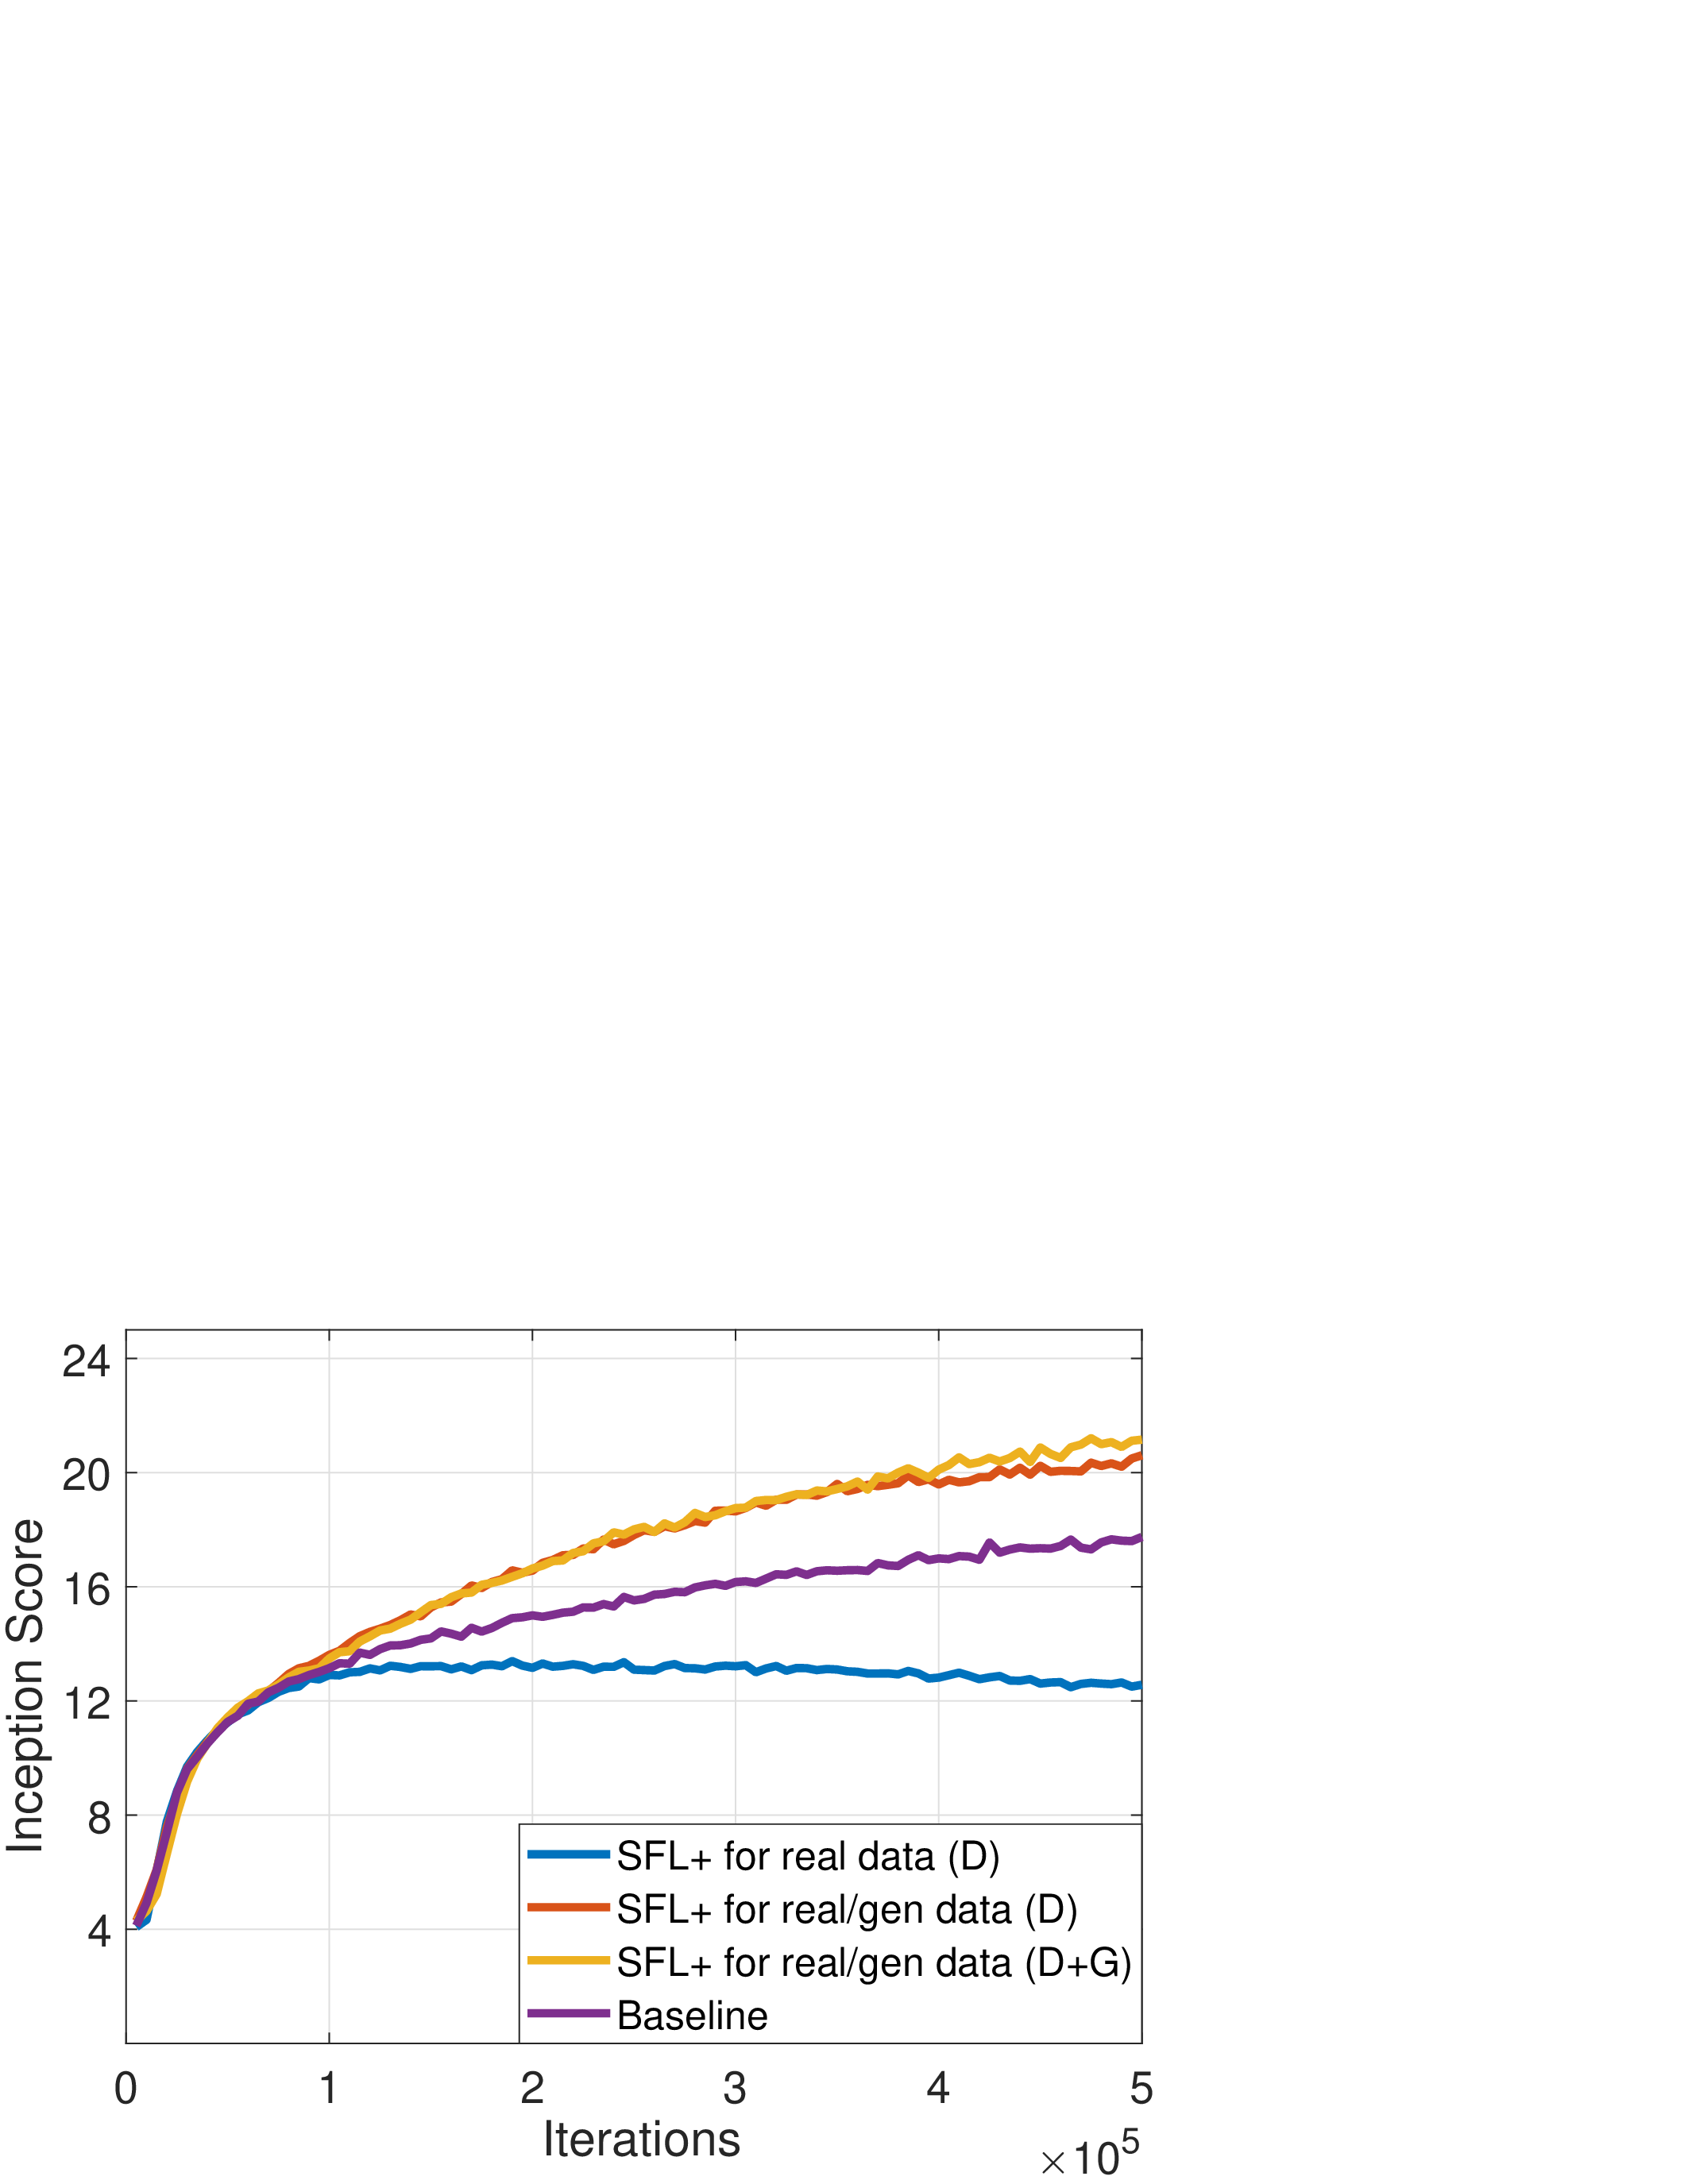}
\label{fig:nrGroup}
}
\subfigure[]{
\includegraphics[width=.6\columnwidth]{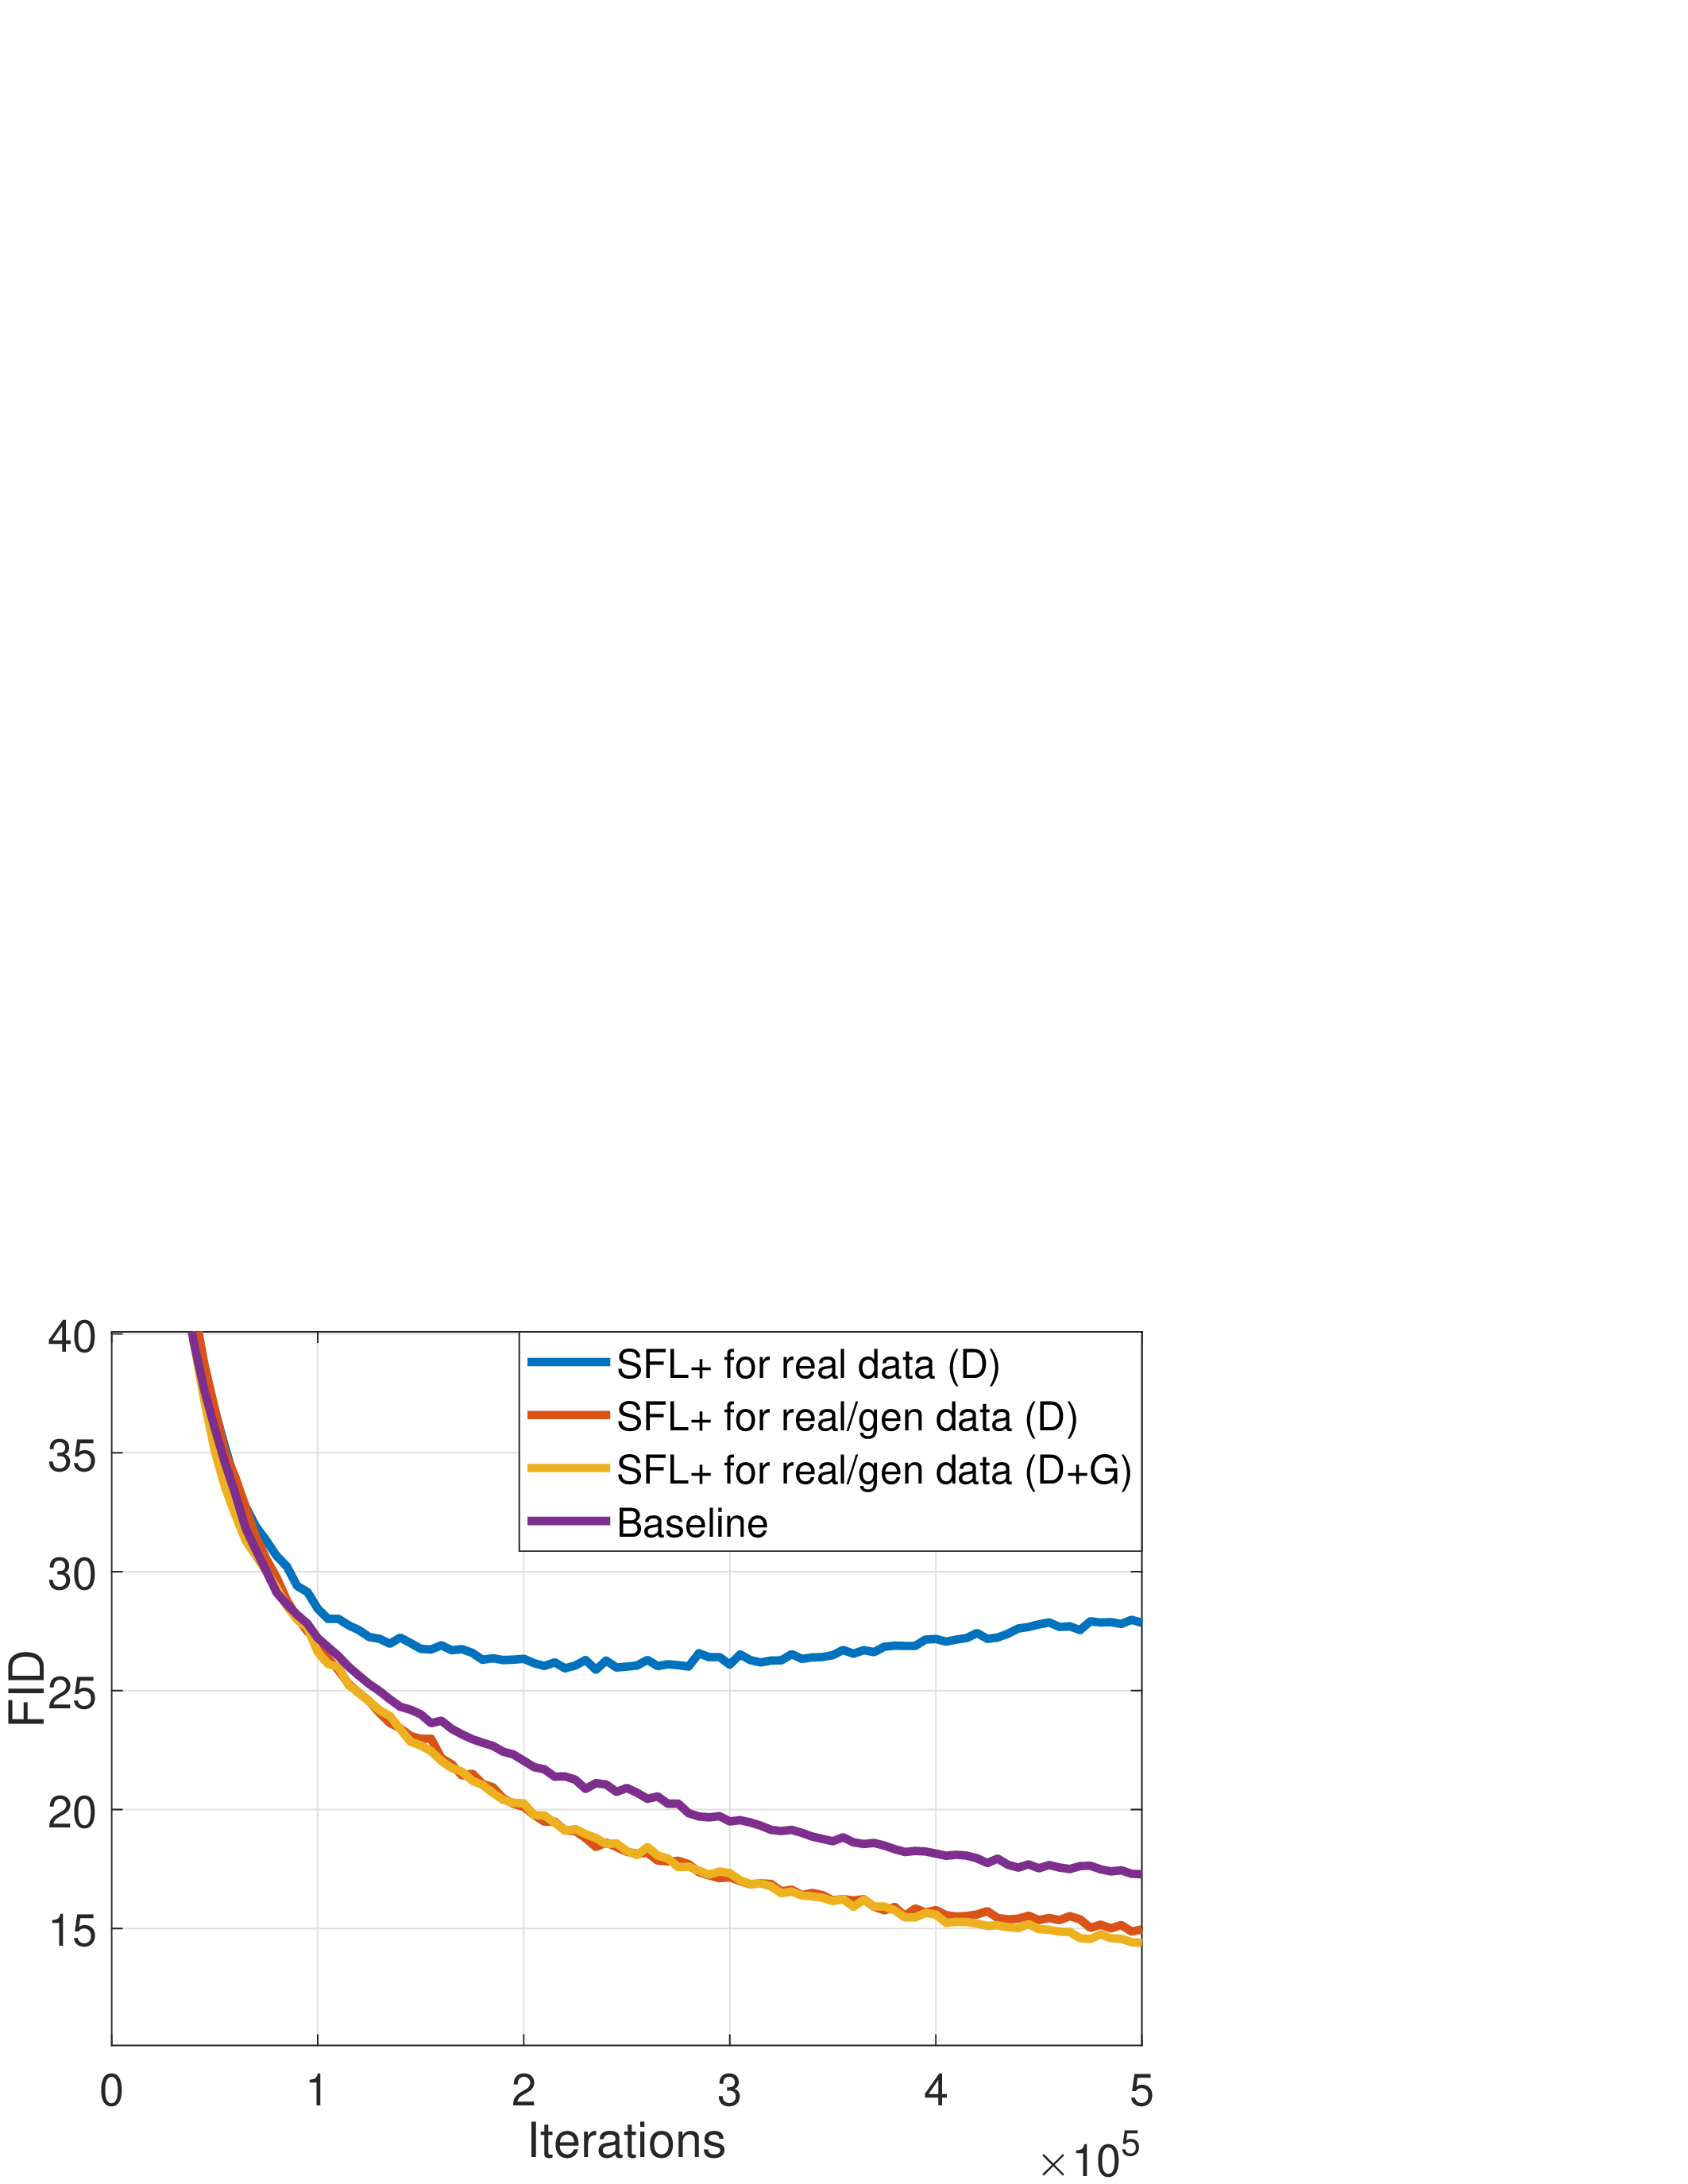}
\label{fig:overallResult}
}
\subfigure[]{
\includegraphics[width=.6\columnwidth]{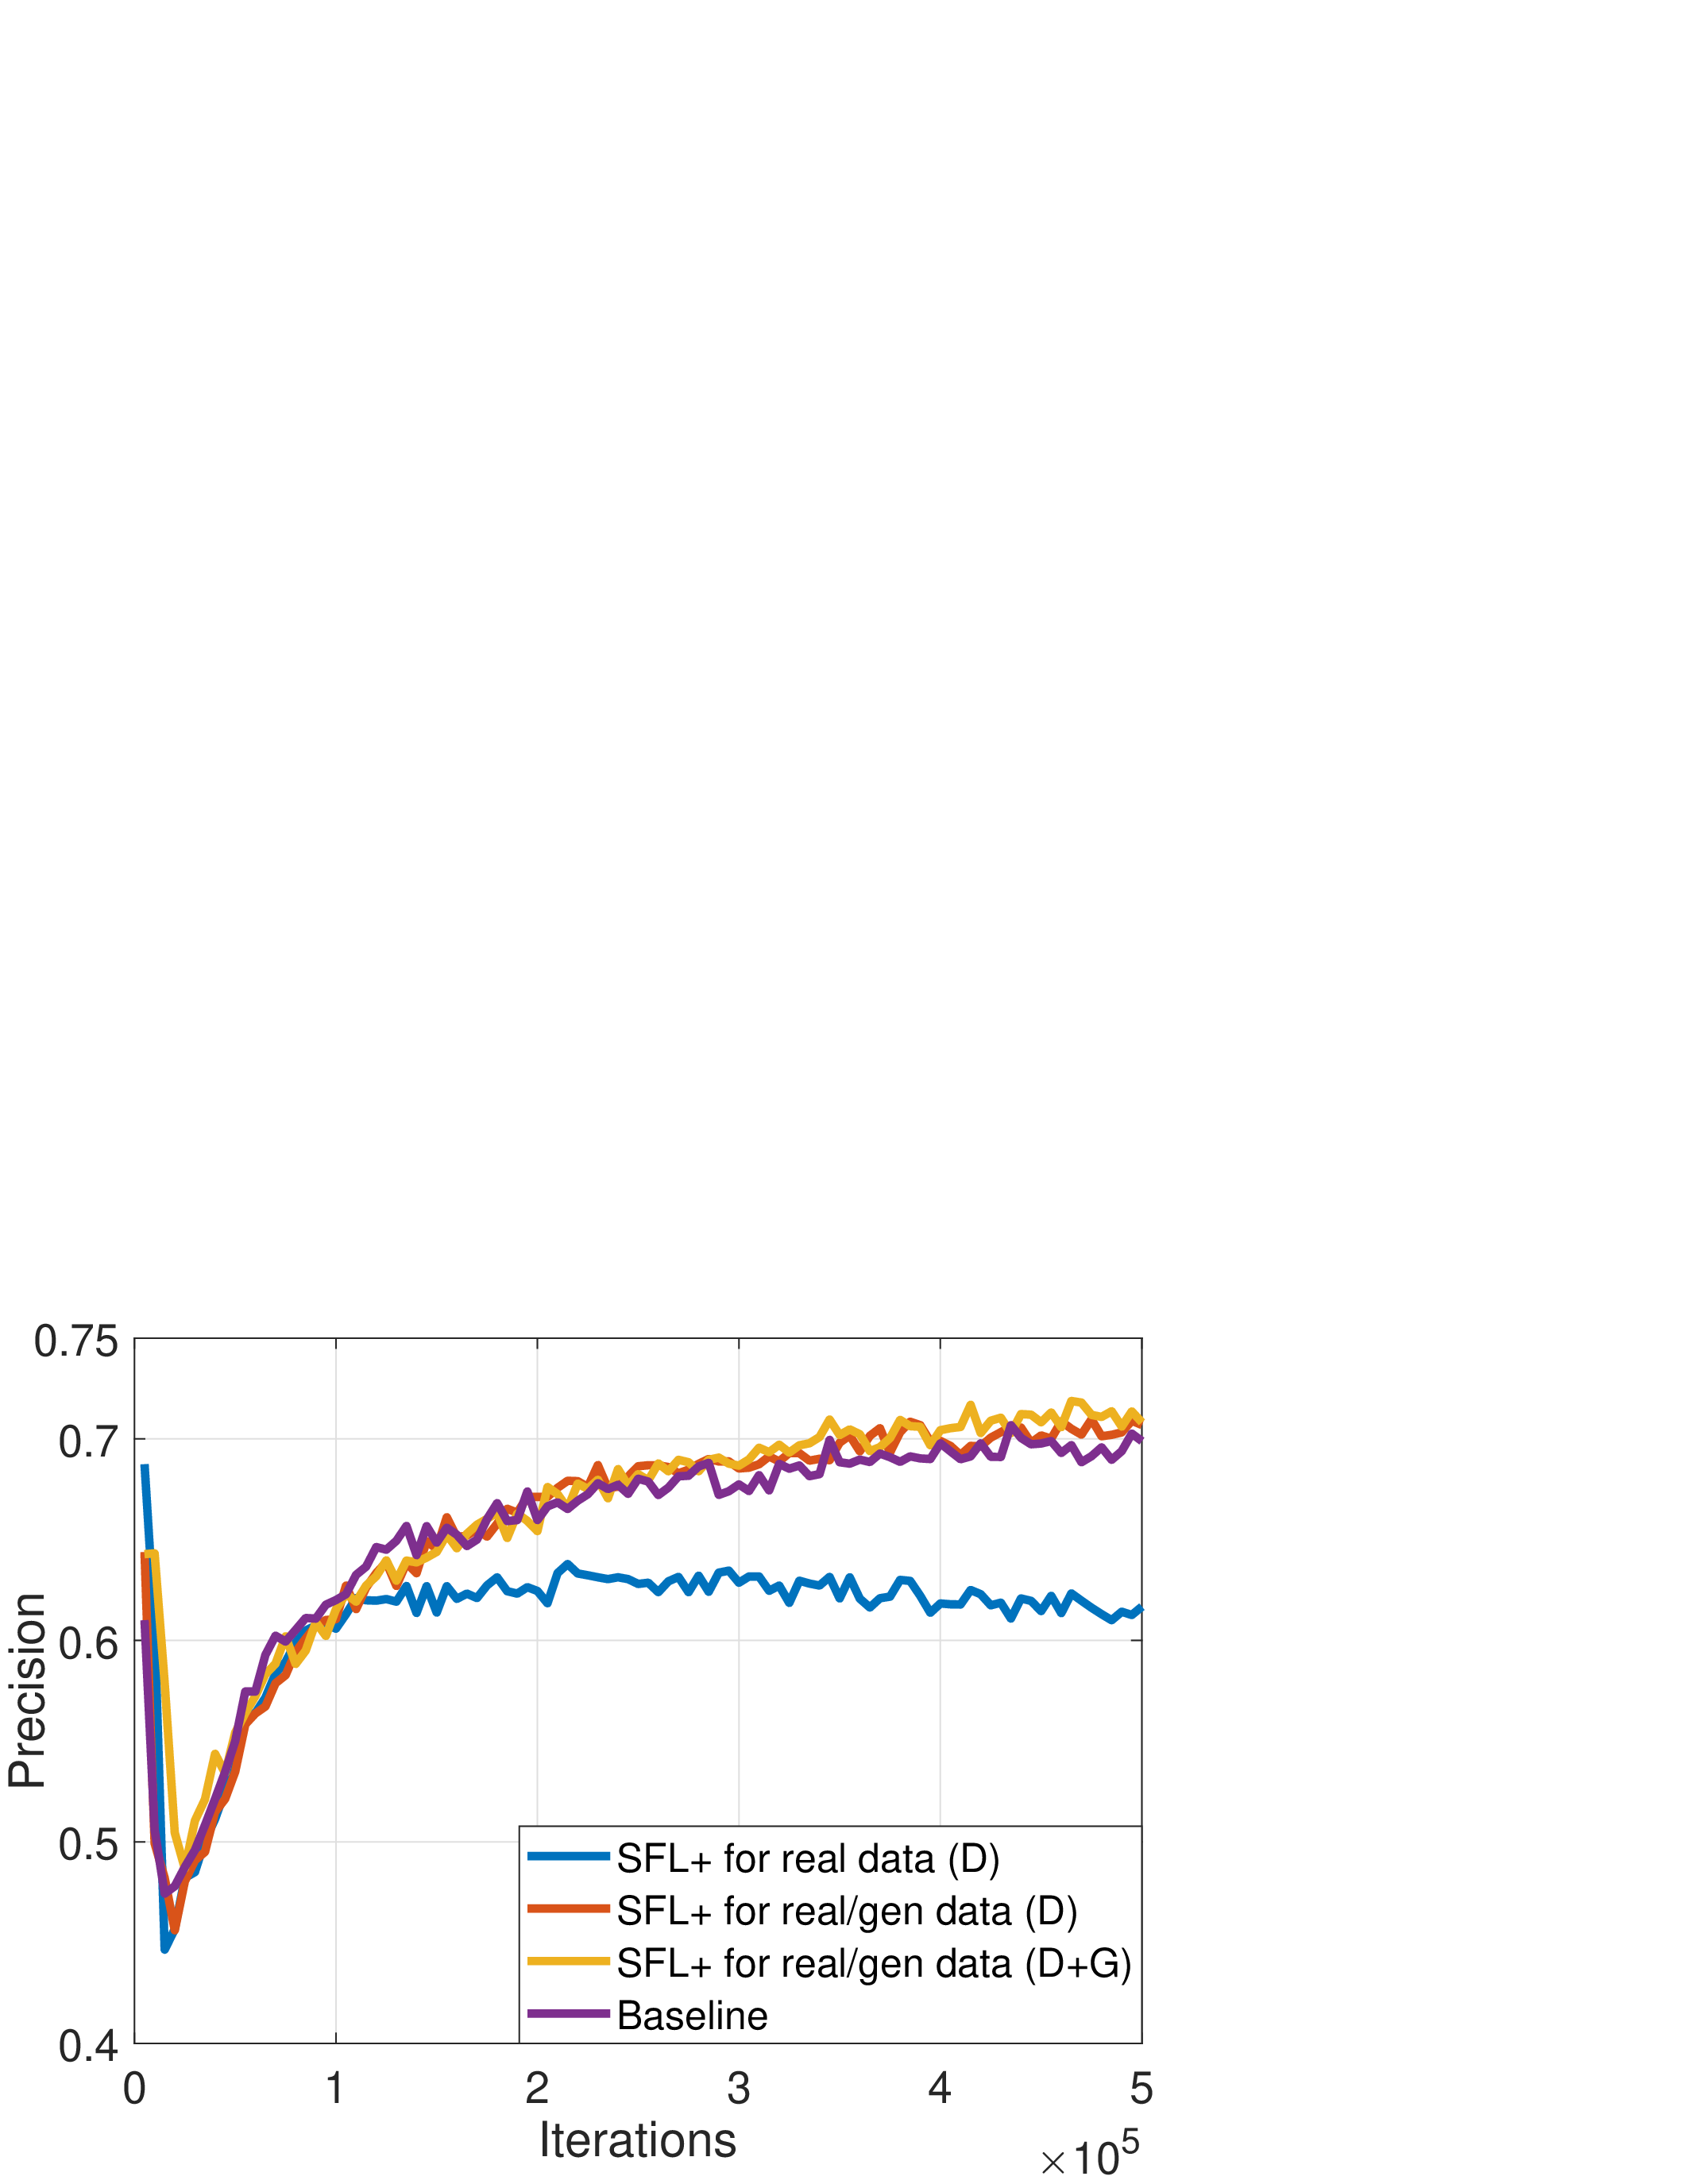}
\label{fig:overallResult}
}
\vskip -0.1in
\subfigure[]{
\includegraphics[width=.6\columnwidth]{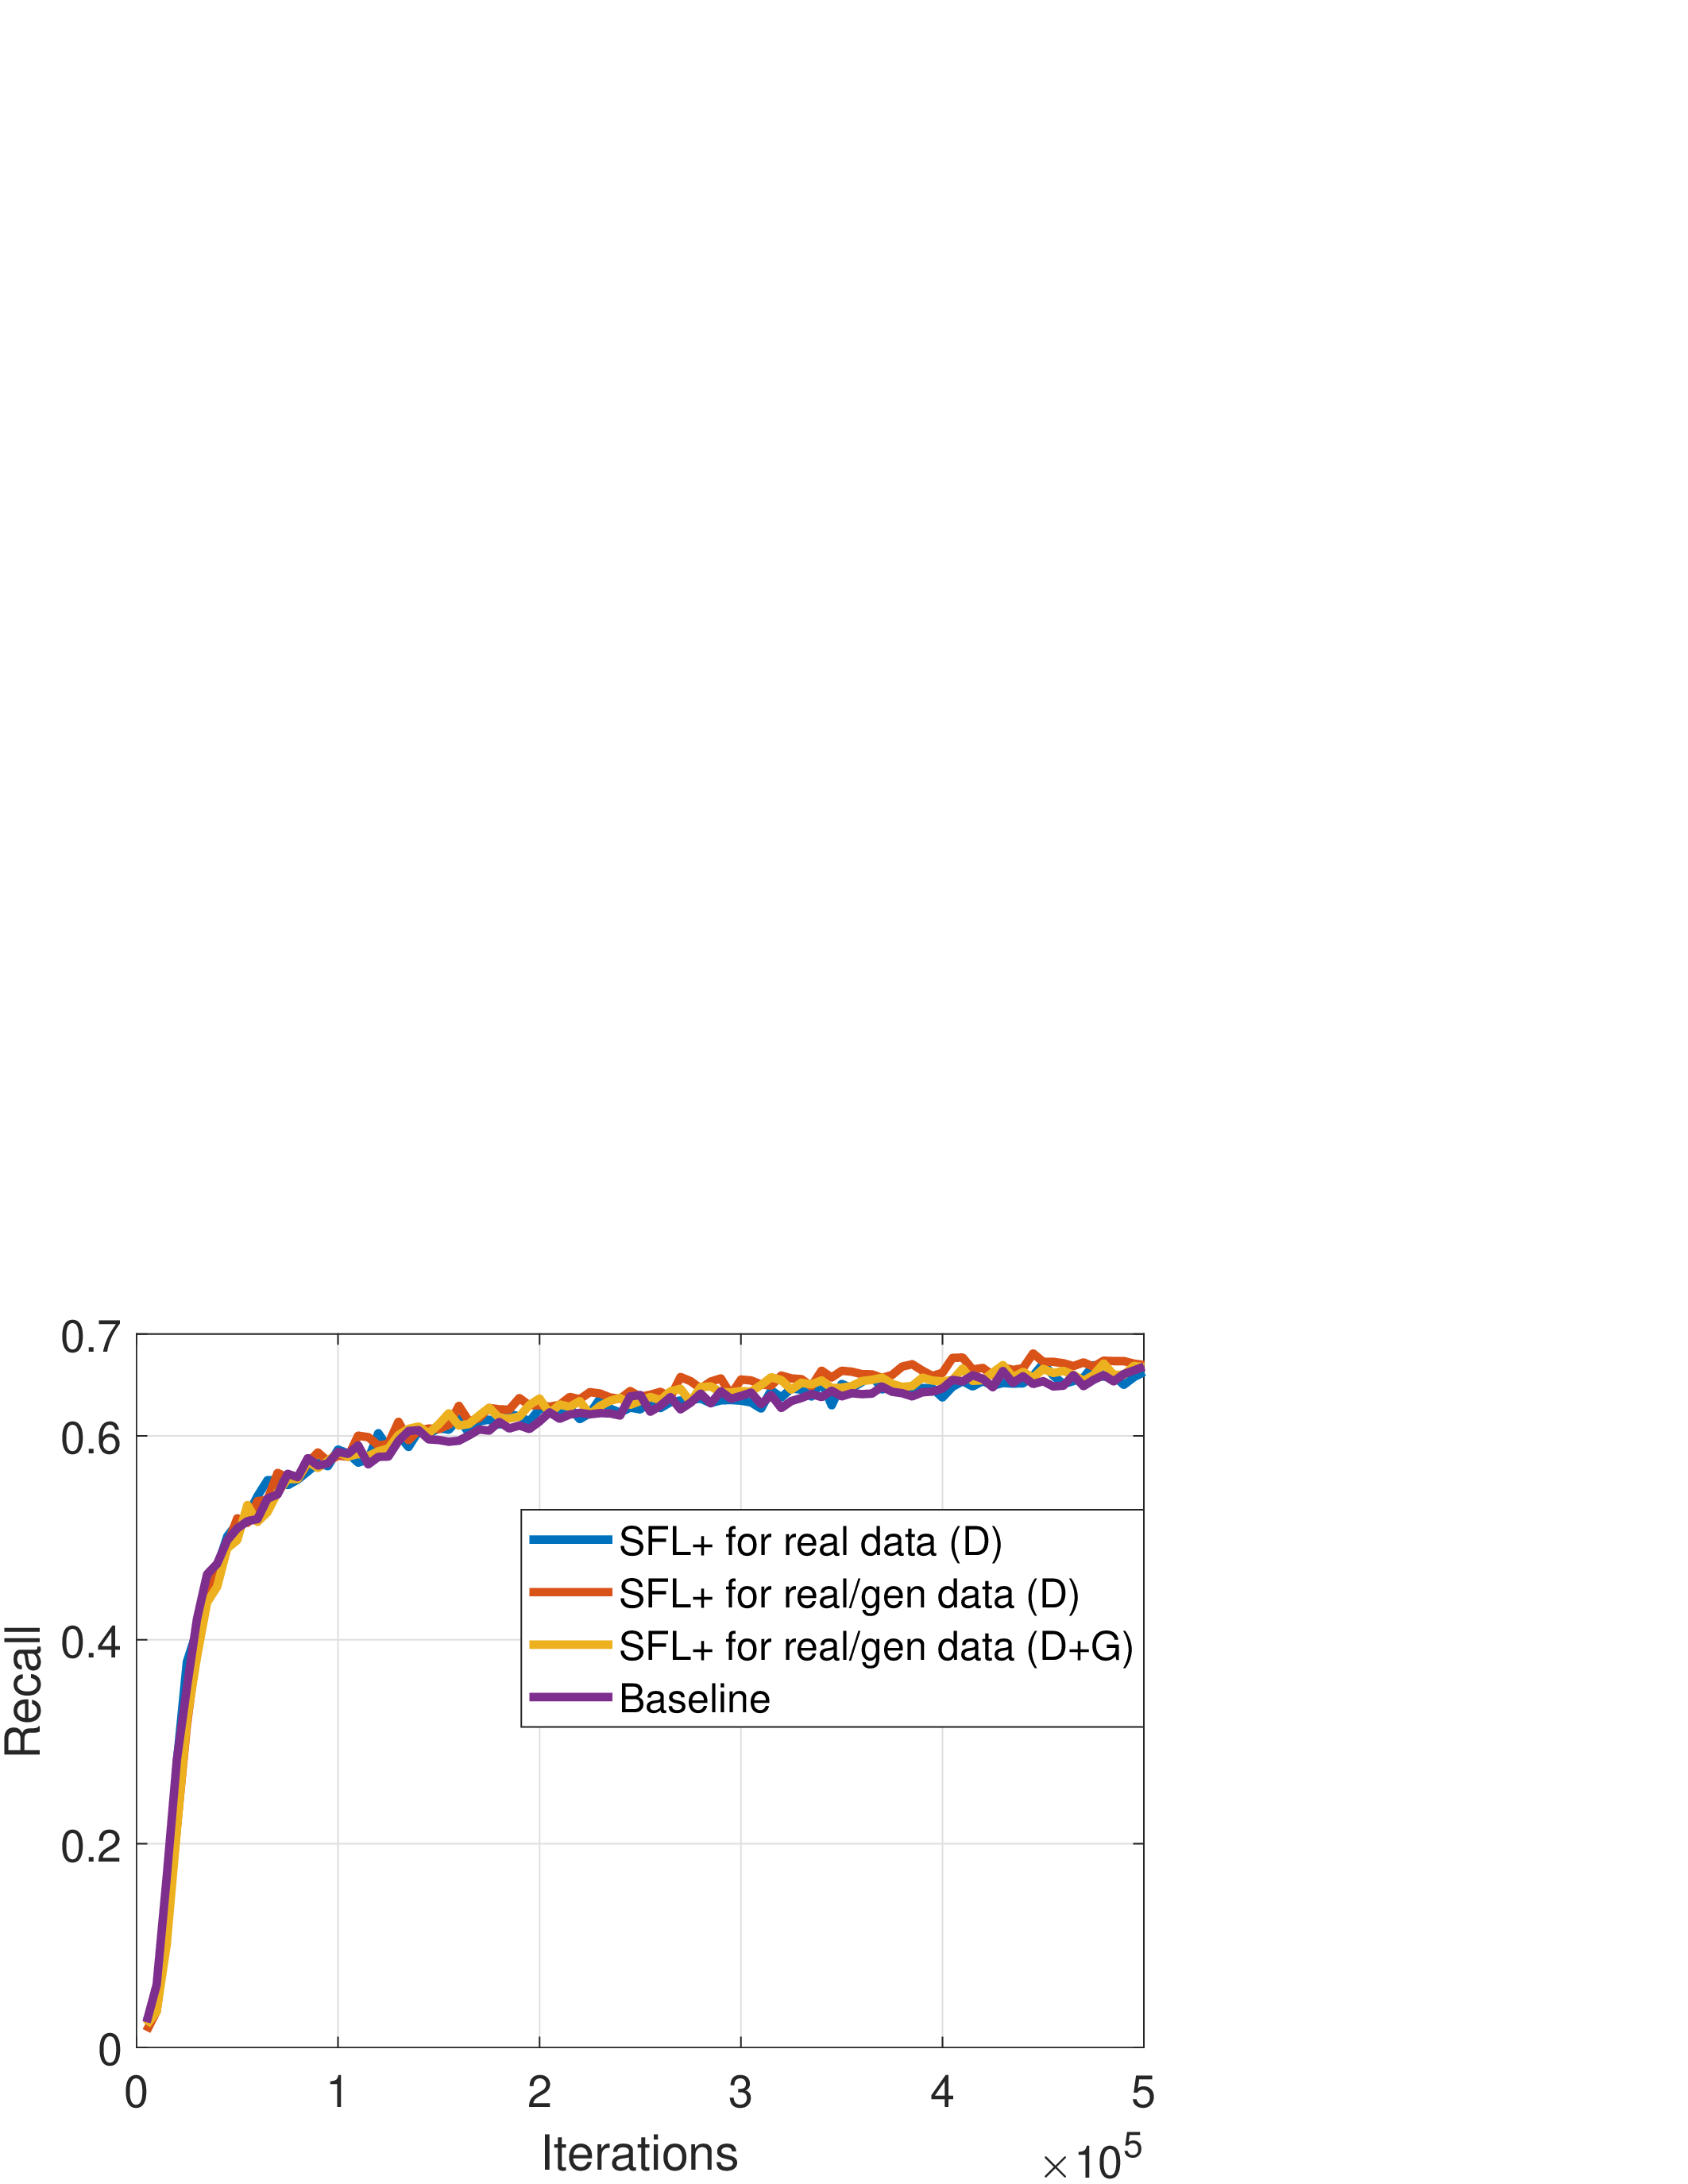}
\label{fig:nrGroup}
}
\subfigure[]{
\includegraphics[width=.6\columnwidth]{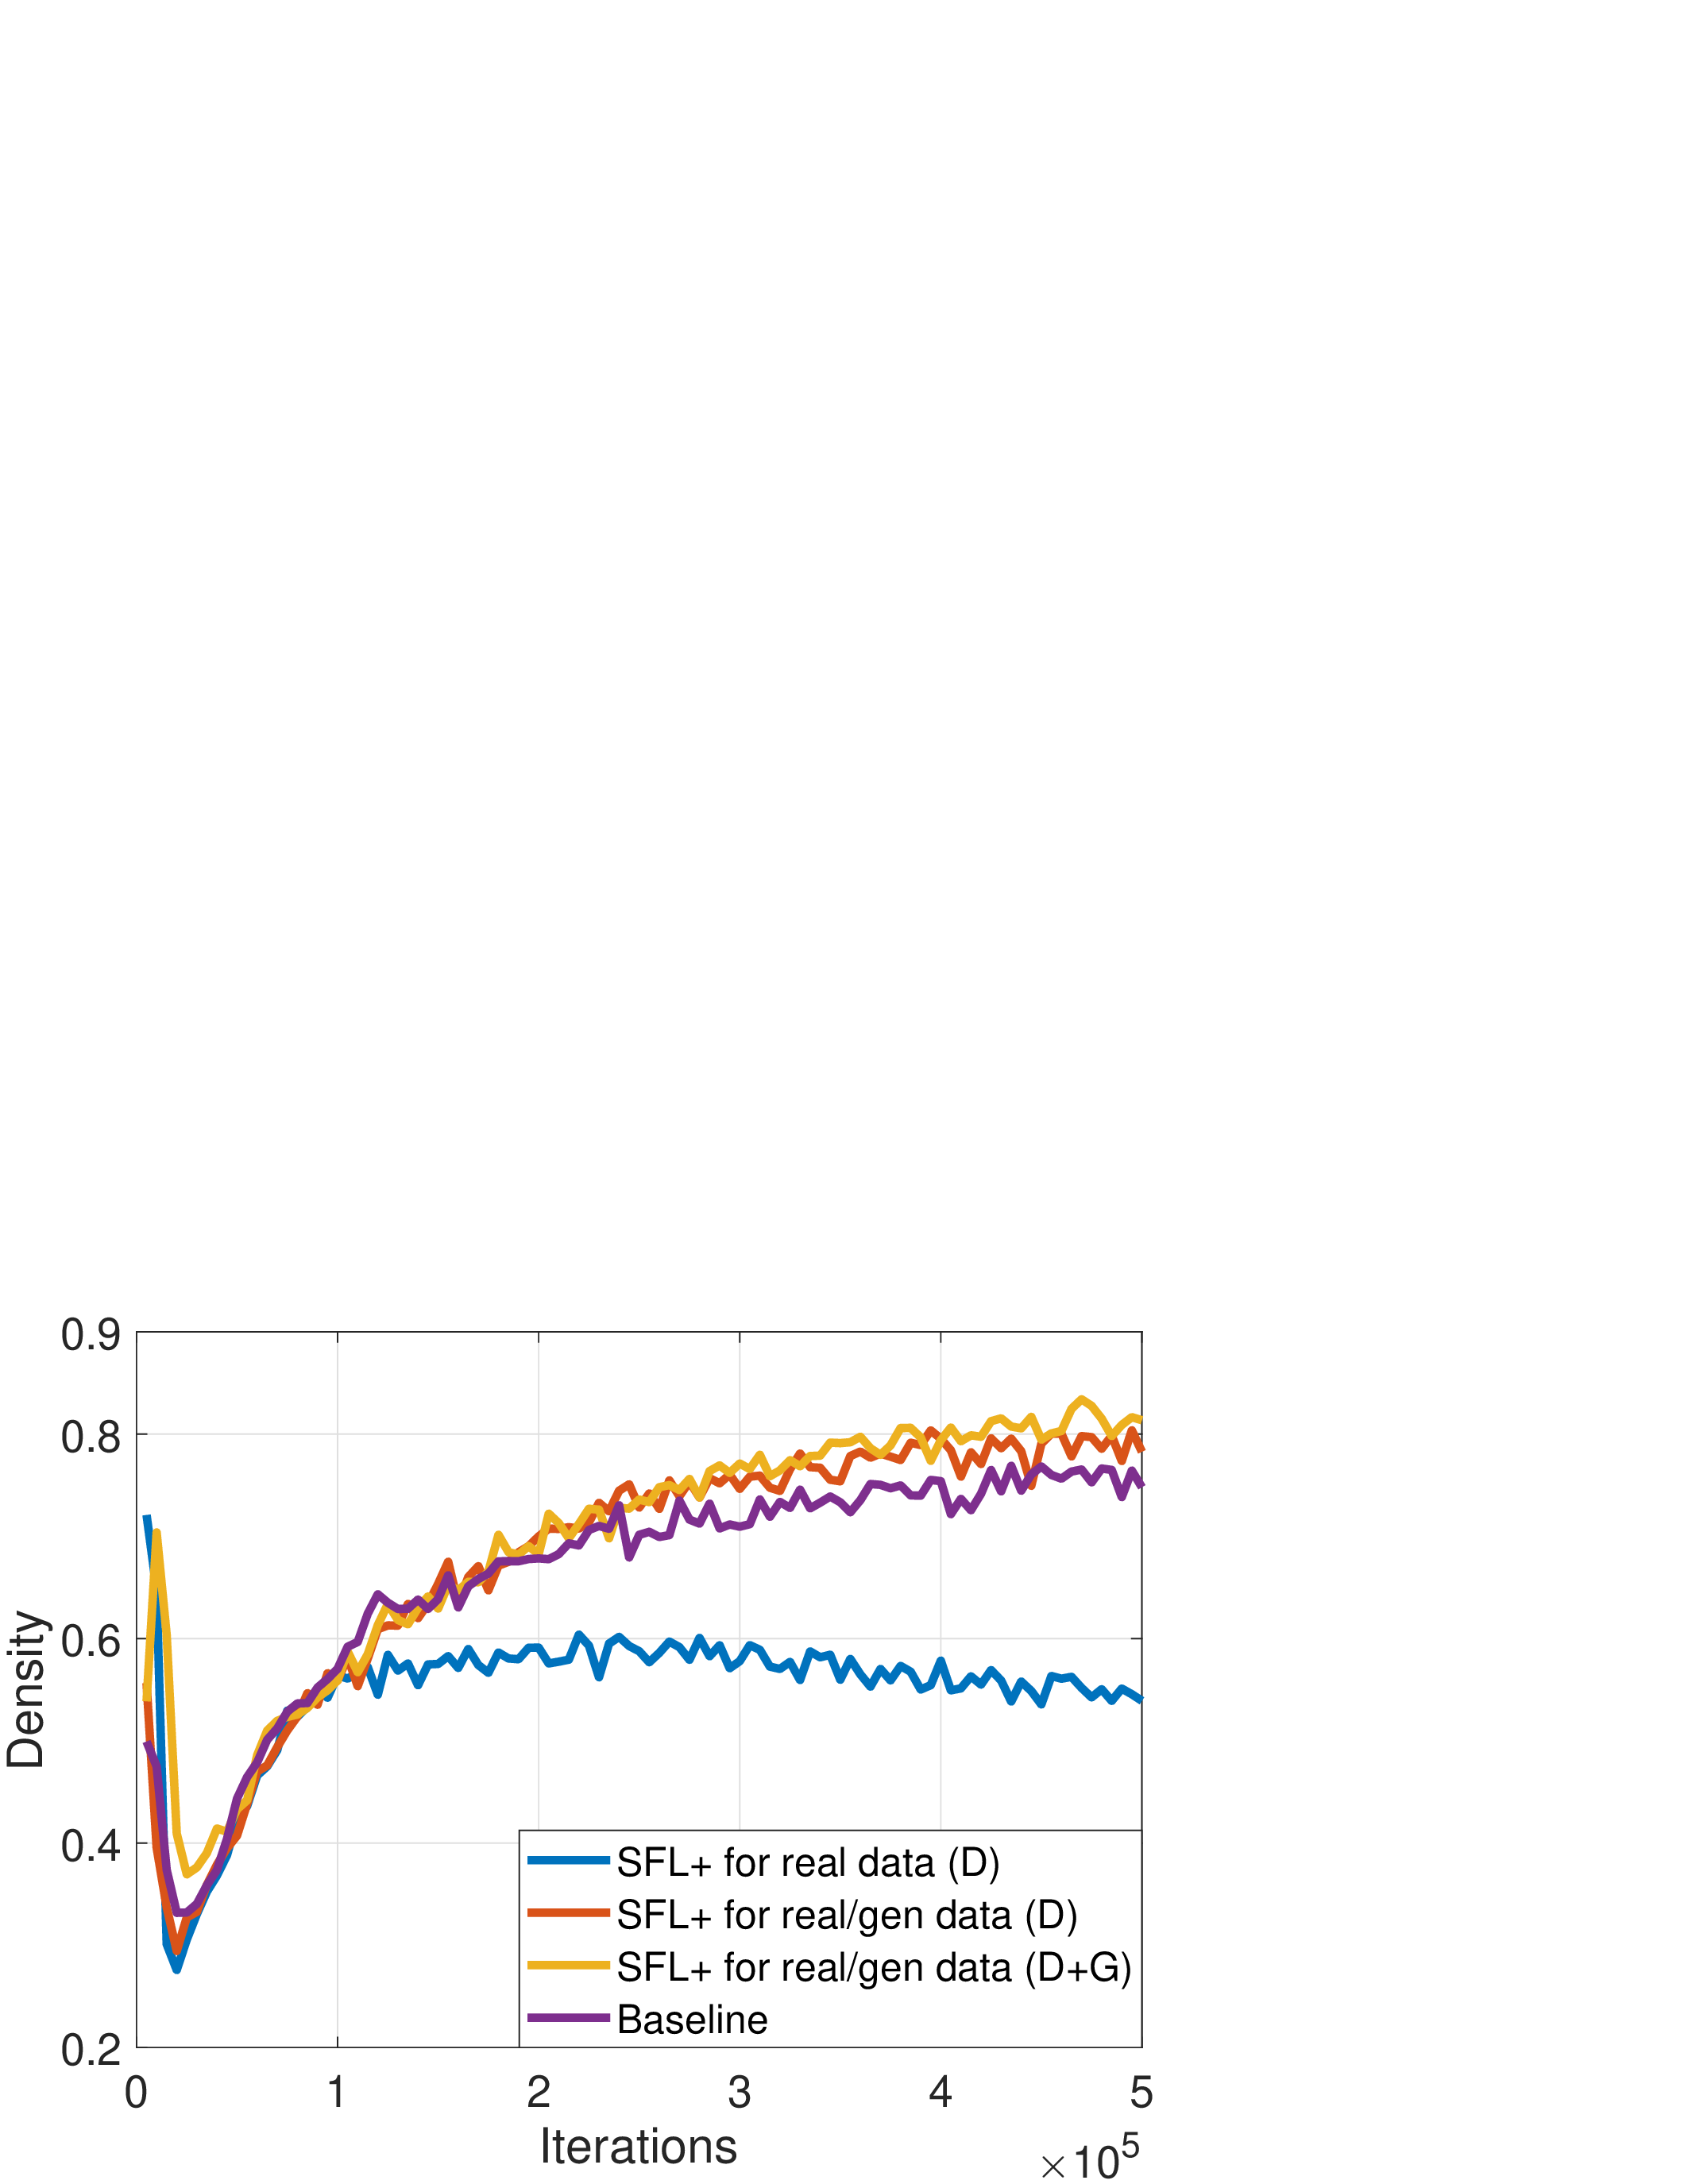}
\label{fig:overallResult}
}
\subfigure[]{
\includegraphics[width=.6\columnwidth]{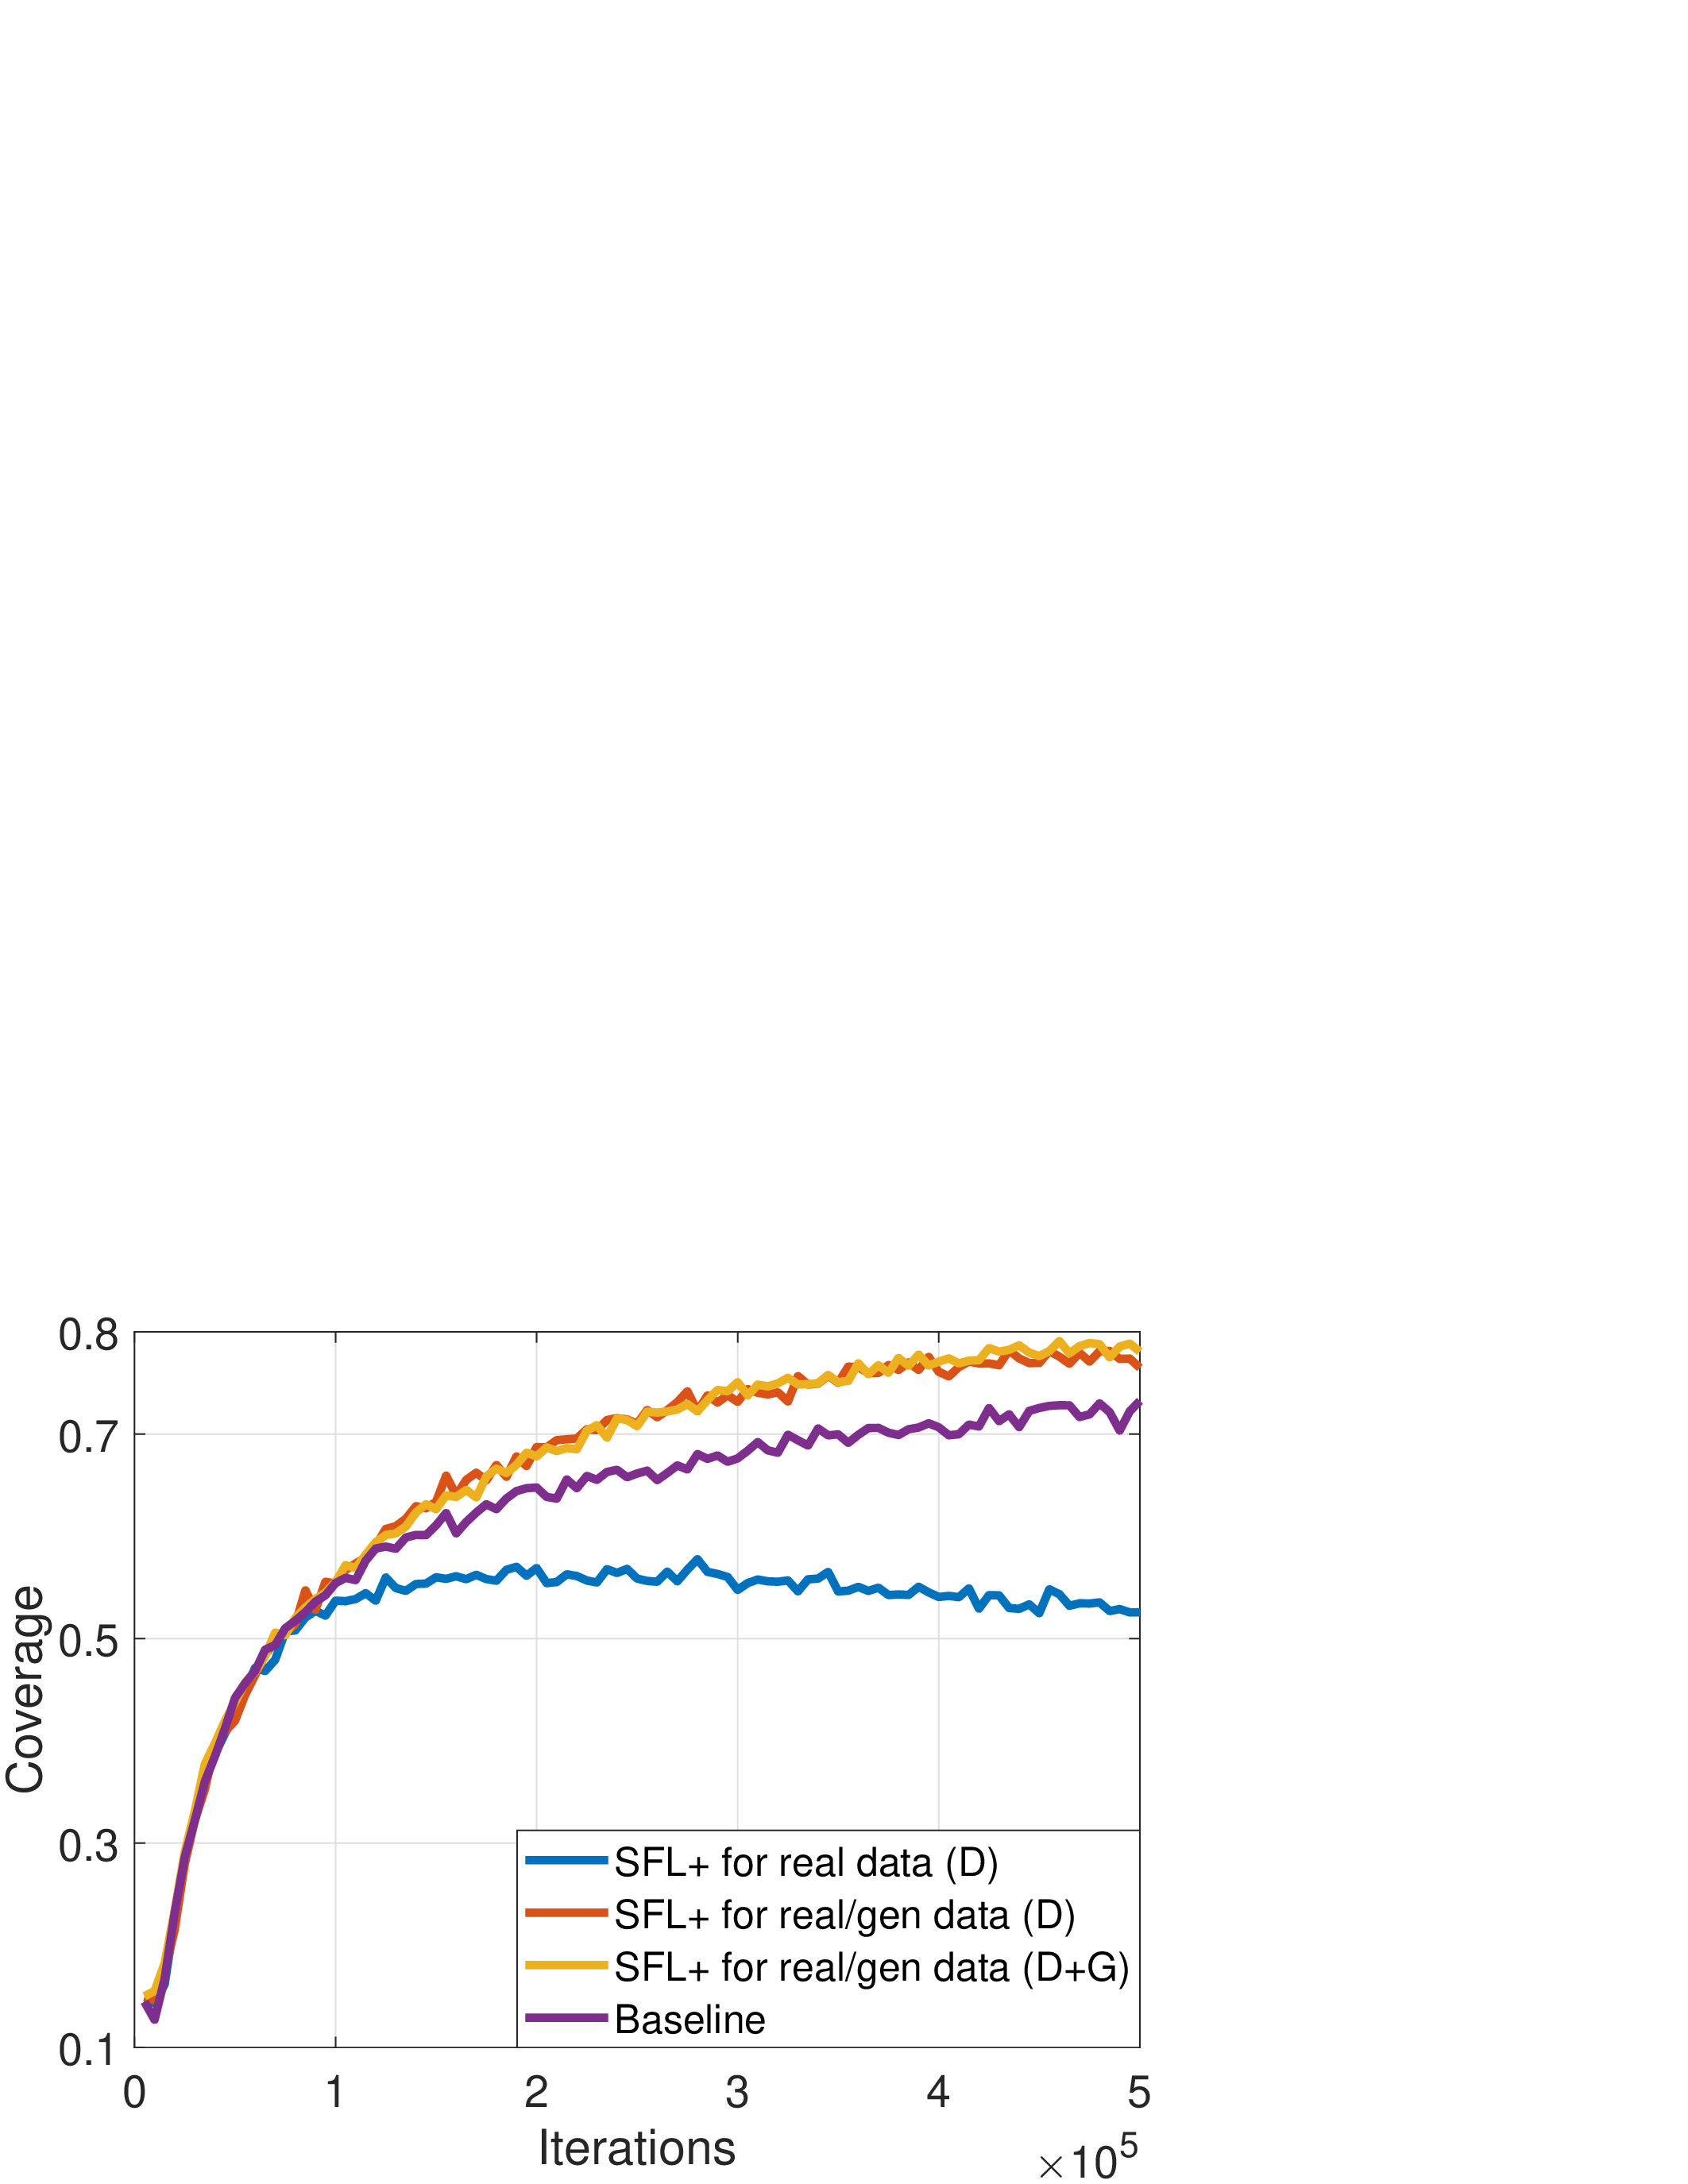}
\label{fig:overallResult}
}
\vspace*{-0.1in}
\caption{
Effect of applying SFL to data and players with SA-GAN in ImageNet $64\times64$. We can achieve the best performance when SFL is applied to the both the discriminator and generator. 
}
\label{supple effect of dtatplayer}
\vspace*{-0.1in}
\end{figure*}

\subsection{CIFAR-100 ($32\times32$)}
We set the maximum FR $\nu$ to $70\%$ ($\gamma=\nu^{(1/E_{max})}=0.7^{(1/500)}$). The remaining parameters are the same as for CIFAR-10. In Table \ref{CIFAR-100}, the SFL BigGAN outperforms the baseline BigGAN in all metrics.

\begin{table}[h]
\vskip -0.1in
\centering
\caption{Comparison using CIFAR-100. We set the maximum focusing range to $70\%$.}
\vspace*{0.1in}
\label{CIFAR-100}
\scalebox{0.9}{
\begin{tabular}{c|cccccc}
\Xhline{2\arrayrulewidth}
              Method   &   IS $\uparrow$    & FID $\downarrow$  & P $\uparrow$  & R $\uparrow$ & D $\uparrow$ & C $\uparrow$ \\ \hline
BigGAN &   9.43   &  8.65     & 0.76 &   0.62  & \textbf{0.97}   &  0.84 \\ 
SFL BigGAN &   \textbf{9.60}   &   \textbf{8.15}     & \textbf{0.77} &  \textbf{0.64}  & \textbf{0.97} &  \textbf{0.87} \\
\Xhline{2\arrayrulewidth}
\end{tabular}}
\vskip -0.1in
\end{table}

\subsection{ImageNet ($128\times128$)}
Due to the limited hardware resources, compared with the full-version BigGAN, we made the following modifications: $bs = 2048$→$bs = 256$, $ch=96$→$ch=64$ and $num\_iters = 500000$. The remaining parameters are the same as for ImageNet ($64\times64$). In Table \ref{ImageNet128}, because we used a smaller batch size ($256$ vs. $1024$) than for FQ-GAN \citep{zhao2020feature}, our baseline achieves worse performance than the baseline$^{\ddagger}$ even when training more iterations ($500k$ vs. $256k$). Despite using $4\times$ a smaller batch size, the SFL+ achieves the best performance for all metrics. We present the generated images for ImageNet ($128\times128$) in Fig. \ref{visualization_SFL_sup_128}.

\begin{table}[h]
\vskip -0.1in
\centering
\caption{Comparison on ImageNet ($128\times128$). Baseline$^{\ddagger}$ and FQ-$256k^{\ddagger}$ were trained for $256K$ iterations with a $1024$ batch size, as quoted in FQ-GAN \citep{zhao2020feature}. The rest of the experiments were conducted with a batch size of $256$ for $500k$ iterations.}
\vspace*{0.1in}
\label{ImageNet128}
\scalebox{0.94}{
\begin{tabular}{c|cccccc}
\Xhline{2\arrayrulewidth}
              Method   &   IS $\uparrow$    & FID $\downarrow$  & P $\uparrow$  & R $\uparrow$ & D $\uparrow$ & C $\uparrow$ \\ \hline
Baseline$^{\ddagger}$ &   63.03   &  14.88     & - &   -  & -   &  - \\ 
FQ-$256k^{\ddagger}$ &   54.36   &  13.77     & - &   -  & -   &  - \\ 
Baseline &   44.29   &  17.55   & 0.75 &   \textbf{0.65}  & 0.90   &  0.75 \\ 
SFL+ &   \textbf{72.76}   &   \textbf{10.34}     & \textbf{0.82} &  \textbf{0.65}  & \textbf{1.17} &  \textbf{0.89} \\
\Xhline{2\arrayrulewidth}
\end{tabular}}
\vskip -0.1in
\end{table}

\begin{figure*}[t]
% \vskip -0.15in
\centering
\subfigure[W/O SFL+]{
\includegraphics[width=0.8\columnwidth]{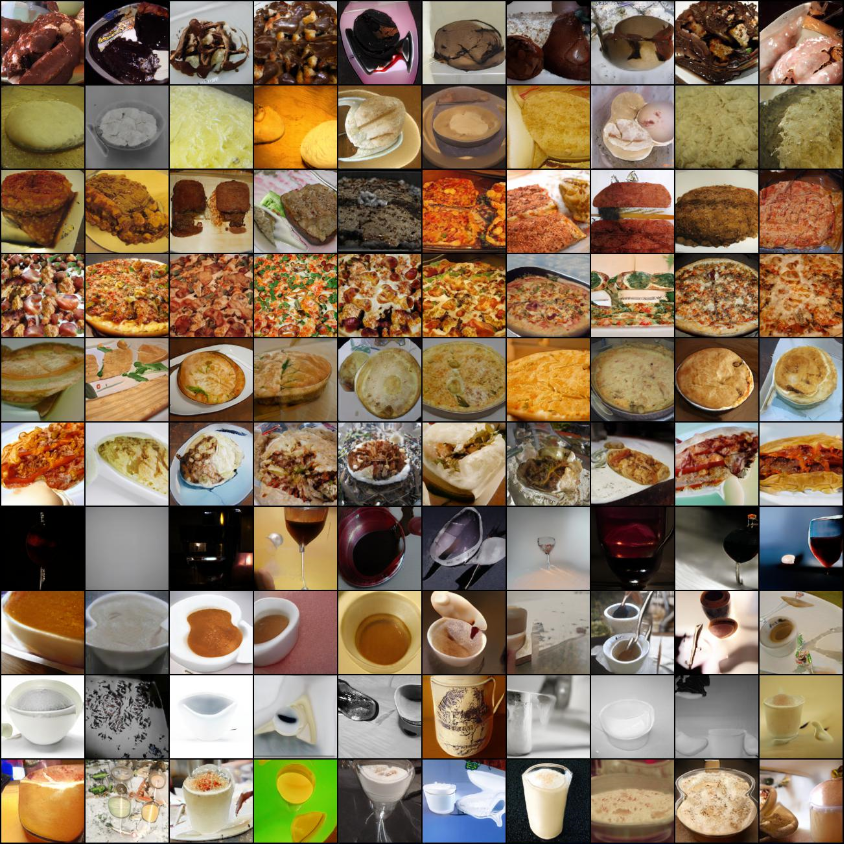}
\label{fig:without SFL}
}
\subfigure[W/ SFL+]{
\includegraphics[width=0.8\columnwidth]{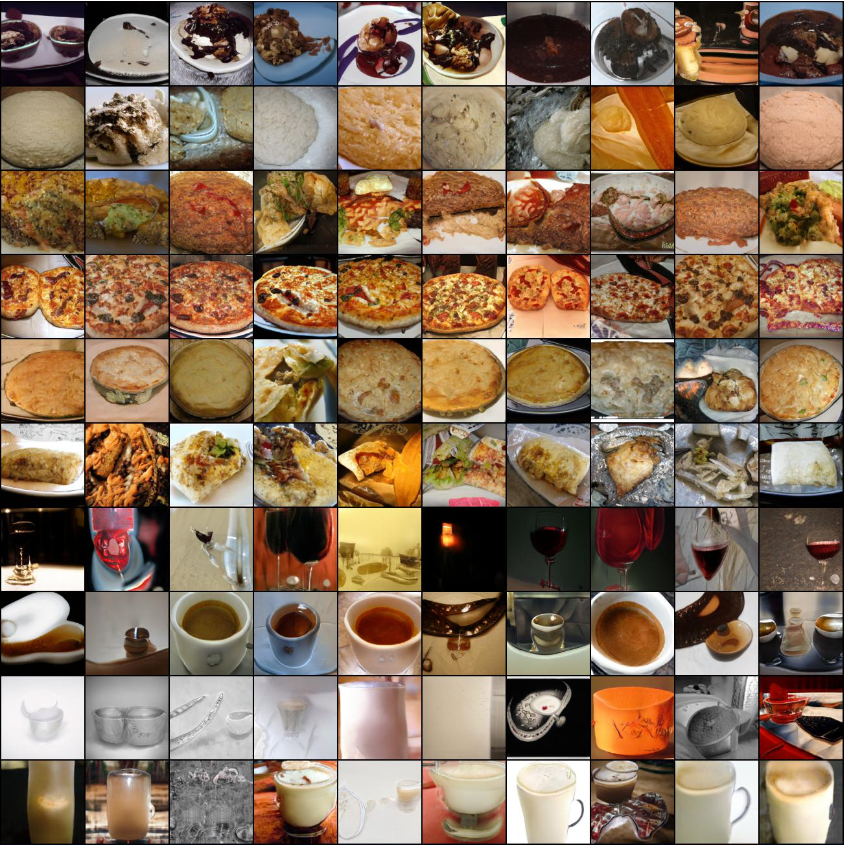}
\label{fig:with SFL}
}
\vskip -0.15in
\subfigure[W/O SFL+]{
\includegraphics[width=0.8\columnwidth]{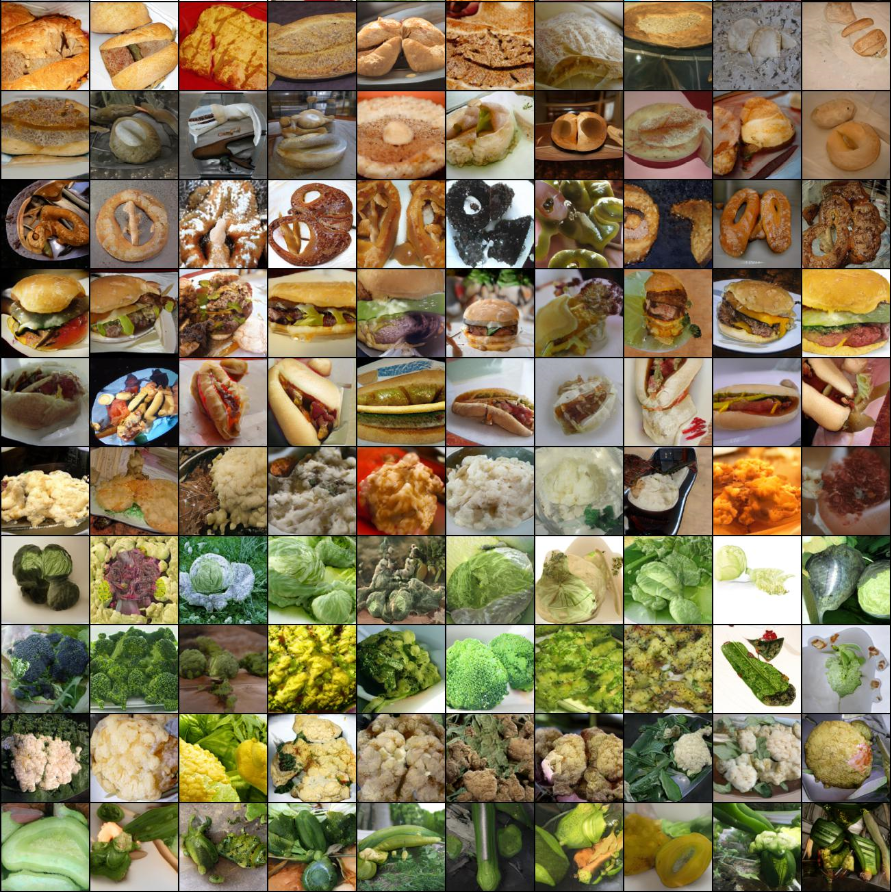}
\label{fig:without SFL}
}
\subfigure[W/ SFL+]{
\includegraphics[width=0.8\columnwidth]{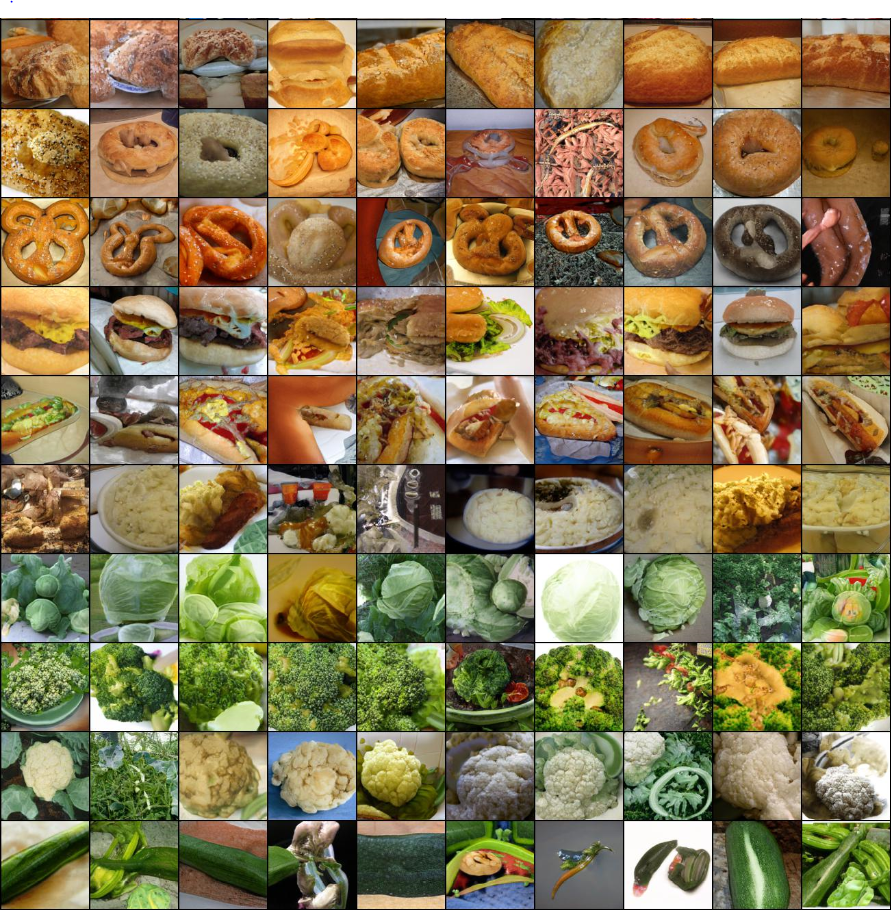}
\label{fig:with SFL}
}
\vskip -0.15in
\caption{
Comparison of generated samples with and without SFL+ on ImageNet $128\times128$. SFL+ effectively learned high quality samples. 
}
\label{visualization_SFL_sup_128}
\vskip -0.2in
\end{figure*}

\subsection{Ablation Study}
We investigated the hyper-parameters of SFL on ImageNet dataset. For all of these experiments, we trained SA-GAN \cite{zhang2019self} to model the ImageNet $64\times64$. Except for the hyper-parameters under consideration, we maintained all settings the same as in Section \ref{Experiments on ImageNet}.

\textbf{Effect of batch size}
Recent works \citep{brock2018large,sinha2020small} suggest that GANs benefit from large batch sizes. To verify the effectiveness of SFL in different batch sizes, we increased  batch size $B$ from $64$ to $256$. In Table \ref{Effect of Batch Size}, the baseline performance gradually improved as the batch size increased, and SFL+ outperformed the baseline model by a significant margin regardless of the batch size.

\begin{table}[H]
\vskip -0.2in
\centering
\caption{Effect of batch size ($B$); SFL+ ($\nu=50$) is applied to SA-GAN on ImageNet $64\times64$ and is effective for different batch sizes for GAN training.}
\vspace*{0.1in}
\label{Effect of Batch Size}
\scalebox{0.9}{
\begin{tabular}{cc|cccc}
\Xhline{2\arrayrulewidth}
\multirow{2}{*}{Metric} & \multirow{2}{*}{Method} & \multicolumn{4}{c}{SA-GAN}                   \\
                  &      & $B=64$   & \multicolumn{2}{c}{$B=128$} & $B=256$   \\ \hline
\multirow{2}{*}{IS $\uparrow$} & Baseline     &  15.19      & \multicolumn{2}{c}{17.77} &   18.54  \\ 
& SFL+     &  \textbf{19.08}      & \multicolumn{2}{c}{\textbf{21.50}} &   \textbf{22.82}   \\ \hline  
\multirow{2}{*}{FID $\downarrow$} & Baseline     &  21.35     & \multicolumn{2}{c}{17.23} &   16.40 \\
& SFL+     &  \textbf{16.98}      & \multicolumn{2}{c}{\textbf{14.20}} &   \textbf{12.94}\\ \Xhline{2\arrayrulewidth}
\end{tabular}}
\vskip -0.2in
\end{table}

\textbf{Effect of maximum focusing rate}
\label{Effect of maximum focusing rate}
Our SFL has only one hyper-parameter; the maximum focusing rate $\nu$. In Table \ref{Effect of Focusing rate}, if we use a too large value of $\nu$, it degrades the performance (especially diversity) by enforcing too many samples as conditional matching. Otherwise, using a too small value for $\nu$ degrades the performance because the effectiveness of SFL+ is reduced. In all cases except $\nu=99$, SFL+ performed better than the baseline (IS: $17.77$, FID: $17.23$).

\begin{table}[H]
\vskip -0.15in
\centering
\caption{Effect of the maximum focusing rate; SFL+ is applied to an SA-GAN on ImageNet $64\times64$ with different $\nu$.}
% \vspace*{0.1in}
\label{Effect of Focusing rate}
\scalebox{0.9}{
\begin{tabular}{c|cccccc}
\Xhline{2\arrayrulewidth}
\multirow{2}{*}{Metric} &  \multicolumn{6}{c}{SA-GAN (\%)}                   \\
                  &   $\nu=99$   & $\nu=70$   & \multicolumn{2}{c}{$\nu=50$} & $\nu=30$  & $\nu=10$   \\ \hline
IS $\uparrow$ &   18.51   &  21.41      & \multicolumn{2}{c}{\textbf{21.50}} &   20.63 & 18.28   \\ 
FID $\downarrow$ &   17.52   &  14.33     & \multicolumn{2}{c}{\textbf{14.20}} &  14.79 &  16.95 \\
\Xhline{2\arrayrulewidth}
\end{tabular}}
\vskip -0.1in
\end{table}

\section{Code Descriptions}
\label{Sup_Code descriptions}
Our code is based on Instance Selection for GANs \citep{devries2020instance}. The change logs are as follows. 
The main change part is the conditional term of the projection discriminator in BigGAN.py (L391-L402, L415-L447). Further, updating the focusing rate is represented in train.py (L66-L71, L146-L155, L185-L209). The SFL and SFL+ are available in Fig. \ref{Code_SFL}.
\begin{figure}[H]
\vskip -0.1in
\begin{center}
\centerline{\includegraphics[width=\columnwidth]{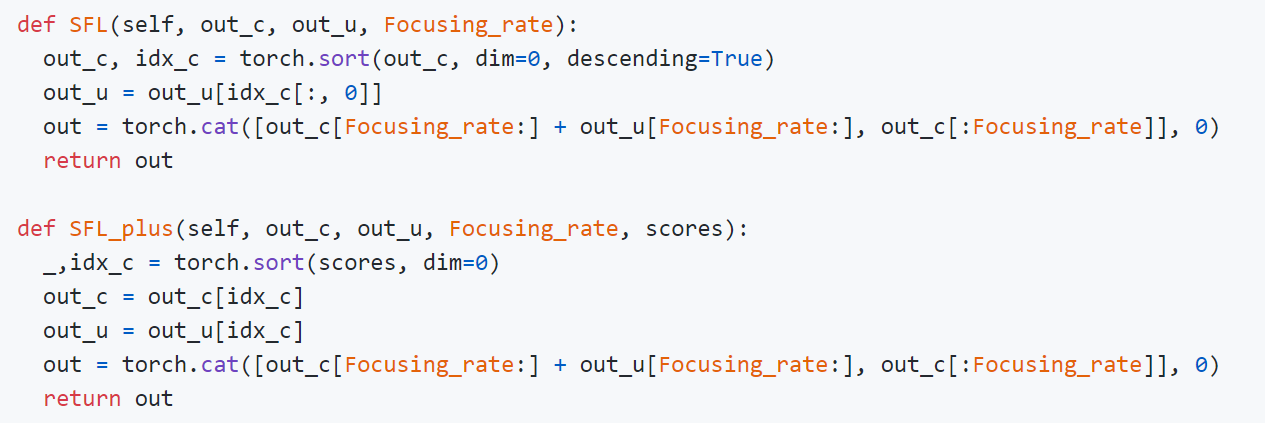}}
\vskip -0.15in
\caption{
SFL in PyTorch. It can be applied to any cGAN using the SFL and SFL_plus functions which are a few lines of code.}
\label{Code_SFL}
\end{center}
\vskip -0.2in
\end{figure}

\section{Detailed Description of Evaluation Metrics}
We used many evaluation metrics to diagnose the effect of training with the proposed method. Each evaluation metric is described in detail. The precision, recall, density, and coverage refer to the description in \citep{naeem2020reliable}.

\subsection{Inception Score (IS)} 
The IS estimates the quality of generated images based on how well Inceptionv3 classifies them. The scores combine both the confidence of the conditional class predictions for each generated image and the integral of the marginal probability of the predicted classes. The major limitation of the IS is that it is insensitive to mode collapse within each class.
% evaluates samples by extracting class probabilities from an ImageNet pretrained Inceptionv3 classifier and measuring the distribution of outputs over all samples. The Inception Score is maximized when a model produces highly recognizable outputs for each of the ImageNet classes. One of the major limitations of the Inception Score is its insensitivity to mode collapse within each class. A model that produces a single high quality image for each category can still achieve a good score.

\subsection{Fréchet Inception Distance (FID)} 
Unlike the earlier IS, which evaluates only the distribution of generated images, the FID compares the distribution of the generated images with the distribution of real images. The FID measures the distance between a generated distribution and real dataset distribution, as approximated by a Gaussian fit to samples projected into the feature space of a pretrained Inceptionv3 model. The FID is defined as follows:
\begin{equation}
\text{FID}:= \left \| m-m_w \right \|_2^2+Tr\left ( C+C_w-2(CC_w)^{1/2} \right )
\label{eq:FID}
\end{equation}
where $m$ and $C$ are the mean and co-variances of the inception embeddings for real-data, and $m_w$ and $C_w$ are the mean and covariance matrices of the inception embeddings for the generated samples. The FID correlates well with image quality, and is capable of detecting mode collapse. However, the FID does not differentiate between fidelity and diversity. Therefore, it is difficult to evaluate whether the model has achieved a good FID score based on good mode coverage, or because it produces high quality samples. 
% As such, it is difficult to assess whether a model has achieved a good FID score based on good mode coverage, or because it produces high quality samples.

\subsection{Precision and Recall (P\&R)} 
The precision and recall were designed to address the limitations of the FID by providing separate metrics to evaluate fidelity and diversity. Precision is described as the percentage of generated samples that fall within the manifold of real images. Recall is described as the percentage of real images which fall within the manifold of generated samples. 
\begin{equation}
\text{Precision}:= \frac{1}{M}\sum_{j=1}^{M}1_{Y_j\in \text{manifold}(X_1,...X_N)}
\label{eq:precision}
\end{equation}
\begin{equation}
\text{Recall} := \frac{1}{N}\sum_{i=1}^{N}1_{X_i\in \text{manifold}(Y_1,...Y_M)}
\label{eq:recall}
\end{equation}
where $X_i$ is a real image, $Y_i$ is a generated image, and $N$ and $M$ are the numbers of real and fake samples. A limitation of the precision and recall is that they are susceptible to outliers in the real and generated distributions.
\subsection{Density and Coverage (D\&C)} 
The practicality of improved precision and recall is still undermined by the vulnerability to outliers and computational inefficiencies. Density and coverage have recently been proposed as robust alternatives to precision and recall. Density improves the precision metric by correcting the manifold overestimation around real outliers. Density is defined as follows:
\begin{equation}
\text{Density} := \frac{1}{kM}\sum_{j=1}^{M}\sum_{i=1}^{N}1_{Y_j\in B(X_i,\text{NND}_k(X_i))},
\label{eq:IS}
\end{equation}
where NND$_k(X_i)$ denotes the distance from $X_i$ to the $k^{th}$ nearest neighbor among \{$X_i$\}, excluding itself. 
Coverage is described as the percentage of real images with a generated sample falling within the manifold. Because the range has fewer outliers, coverage improves the recall metric to better quantify this by building the nearest neighbor manifold around the real sample instead of the fake sample. Coverage is defined as follows:
\begin{equation}
\text{Coverage} := \frac{1}{N}\sum_{i=1}^{N}1_\exists_{j \text{ s.t } Y_j\in B(X_i,\text{NND}_k(X_i))}.
\label{eq:IS}
\end{equation}
%8. applications -> 경훈
%1. Network architecture -> 경훈    biggan, sagan

%5. 128x128

%A. BigGAN
%A.1. More results on Ablation Study
%In Figure 8, we provide the detailed learning curves under different FQ settings on CIFAR100.
%A.2. Experiment setup
%• CIFAR-10 and CIFAR-100 (32 × 32 ): bs = 64, ch =64. The architecture is given in Table 8. Parameters are set as: bs = 64, G lr = 2e−4, D lr =2e−4, D step = 4, G step = 1. To get the best results shown in Table 2, we set P = 10, λ = 0.9, α = 1.0 of FQ being added at the layers [0, 1, 2, 3].
%• ImageNet (64 × 64): bs = 512, ch = 64. The architecture is the same as that in Imagenet (128 × 128) when you omit the bottom downsample ResBlock in the discriminator and the top upsample ResBlock in the generator, as shown in Table. 10. Parameters are set as: bs = 512, G lr = e−4, D lr = 4e−4, D step =1, G step = 1 with self-attention at resolution 32×32. P = 10, λ = 0.7, α = 1.0 of FQ.

%Hinge loss, DC loss 설명
